# Supplementary material for: Correlation of the Superconducting Critical Temperature with Spin and Orbital Excitation Energies In (Ca{x}La{1-x})(Ba{1.75-x}La{0.25+x})Cu{3}O{y} as Measured by Resonant Inelastic X-ray Scattering
Source: arXiv:1508.02021 ancillary file (2015-08-09)

# Supplementary Materials

These Supplementary Materials are a display of all the fitting curves for each spectra at each $q$ position, using the methods described in the main text. They are arranged into sections in the following pages (1) Undoped (UD) magnon spectra (2) Optimally doped (OD) magnon spectra (3) Undoped *dd* excitation spectra.

The energy scale originally used during the fitting, whose graphs are displayed here, was multiplied by -1 with respect to what is used in the main text, but the direction of increasing energy transfer on the graphs, which is to the left, are the same as used in the main text.

As an alternative to the in-plane momentum transfer $q$, the angle $D$ of the sample's $c$-axis from specular reflection condition (with negative $D$ closer to grazing incidence; the geometry is shown in the figure below) , in units of degrees, is specified on each graph. The relation between $D$ and $q$, is given by the formula $q = \left(\frac{2a}{13.3137}\right) \cdot \cos(25°) \cdot \sin(D)$ (for 932 eV beam energy used)

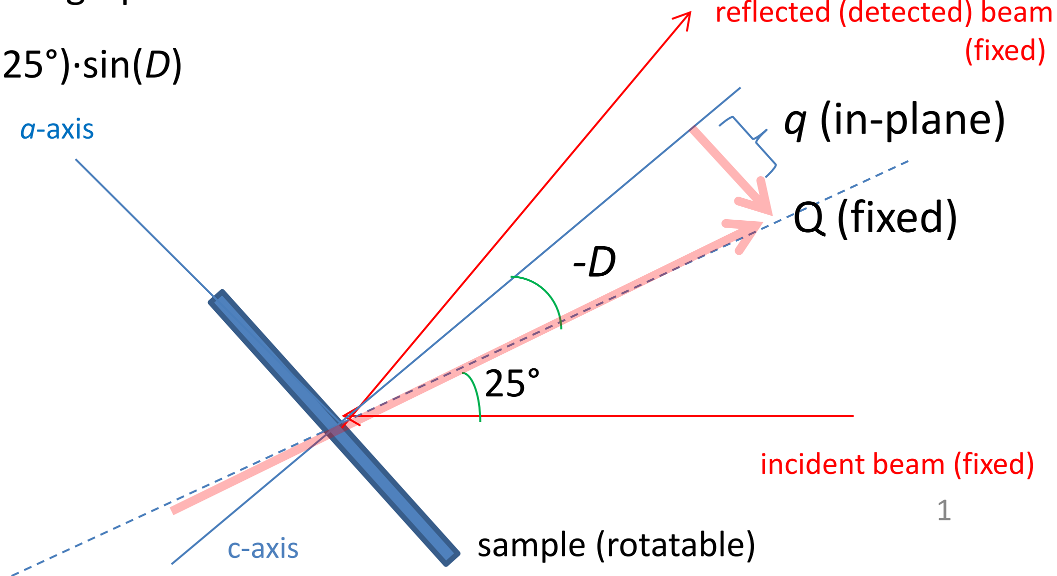

# 1. Undoped Samples : Magnon fits

These are arranged in four *D*-positions (*q*-positions) per page, as per the template :

| | |
|---|---|
| D1 σ(vertical)-polarized<br>D1 π(horizontal)-polarized | D3 σ(vertical)-polarized<br>D3 π(horizontal)-polarized |
| D2 σ(vertical)-polarized<br>D2 π(horizontal)-polarized | D4 σ(vertical)-polarized<br>D4 π(horizontal)-polarized |

The raw data , background from *dd* tails, 1-magnon,2-magnon and 0.8 eV peak (if included in the fit), as well as total fit are shown. The quasielastic component is not shown to simplify the graphs, but its contribution is clear from the raw data combined with the other fit components.

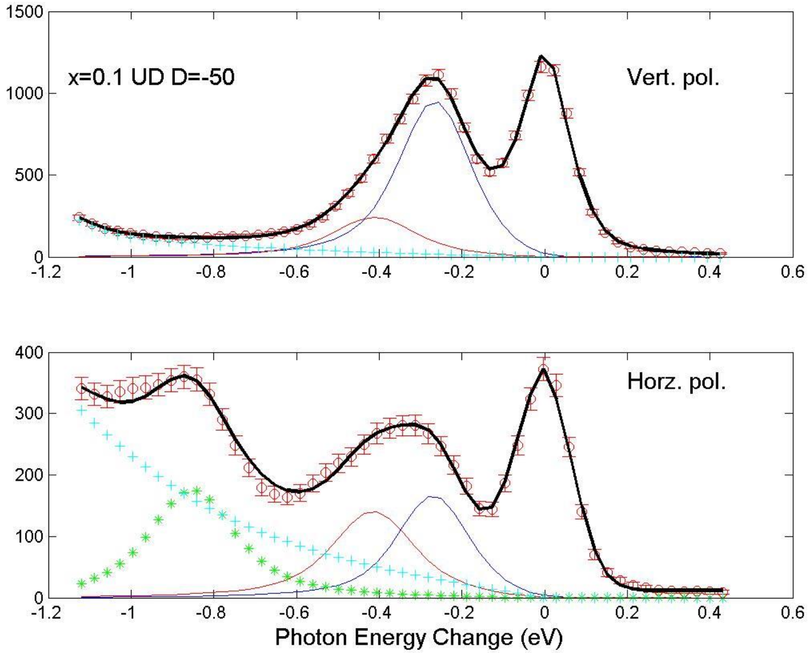
x=0.1 UD D=-50
Vert. pol.
Horz. pol.
Photon Energy Change (eV)

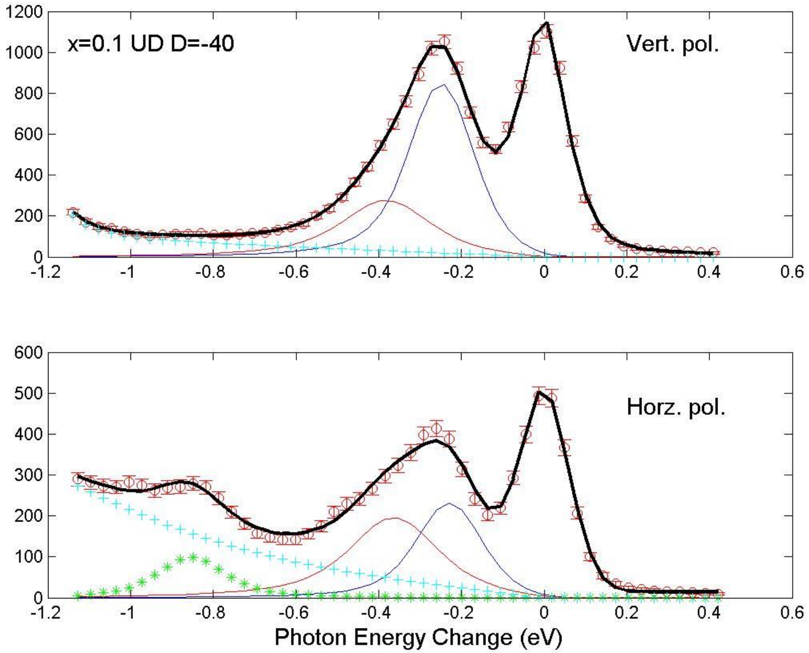
x=0.1 UD D=-40
Vert. pol.
Horz. pol.
Photon Energy Change (eV)

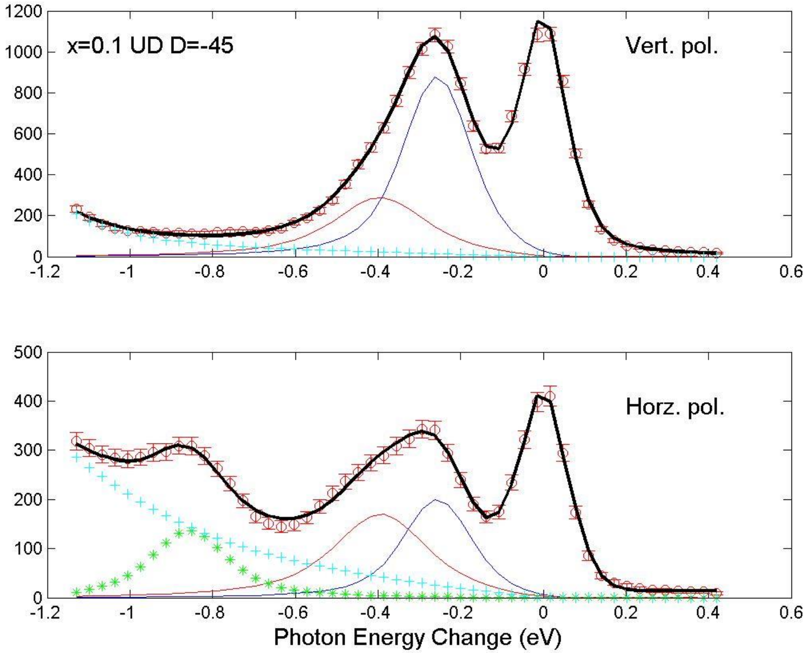
x=0.1 UD D=-45
Vert. pol.
Horz. pol.
Photon Energy Change (eV)

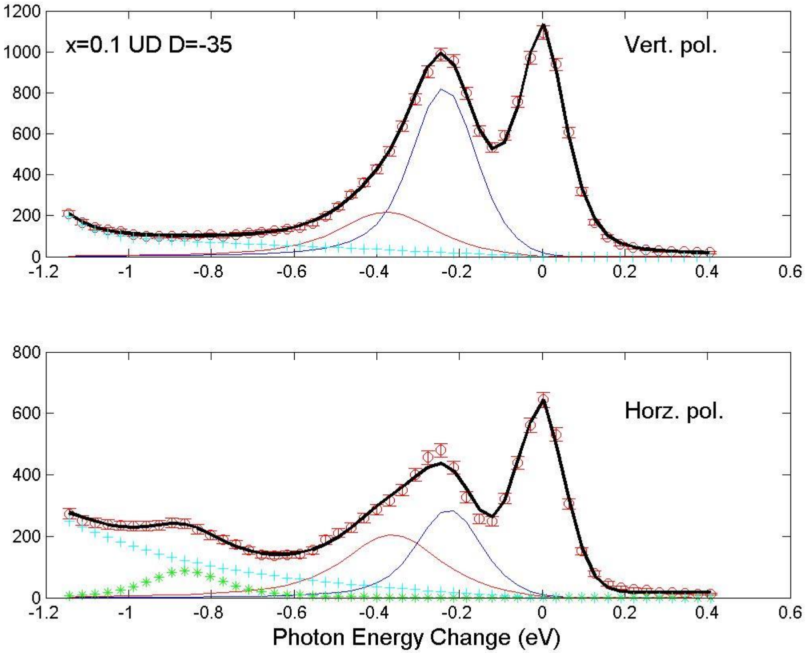
x=0.1 UD D=-35
Vert. pol.
Horz. pol.
Photon Energy Change (eV)

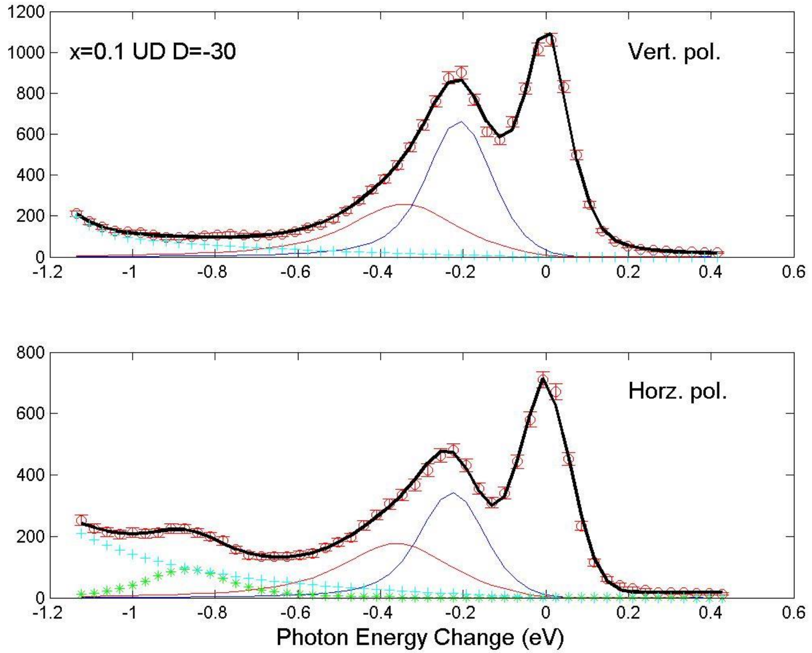
x=0.1 UD D=-30
Vert. pol.
Horz. pol.
Photon Energy Change (eV)

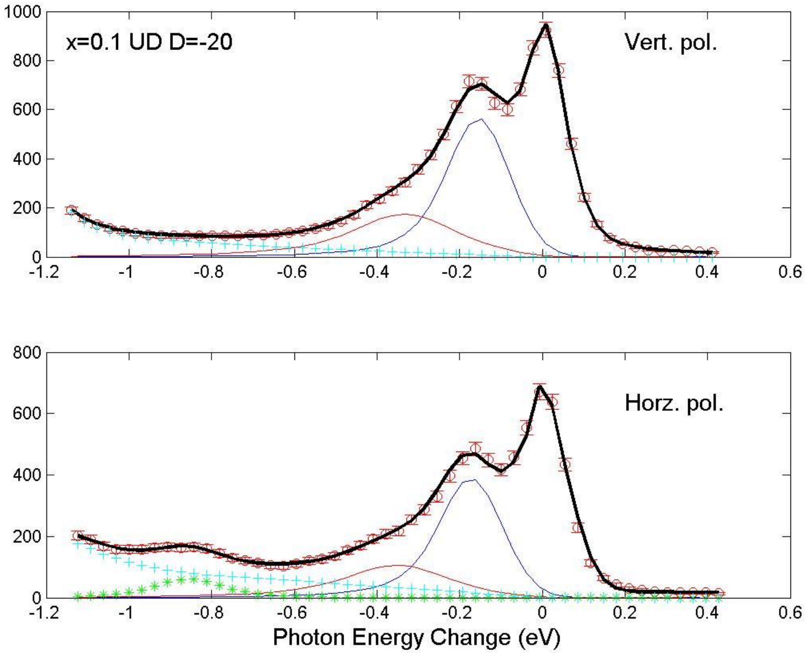
x=0.1 UD D=-20
Vert. pol.
Horz. pol.
Photon Energy Change (eV)

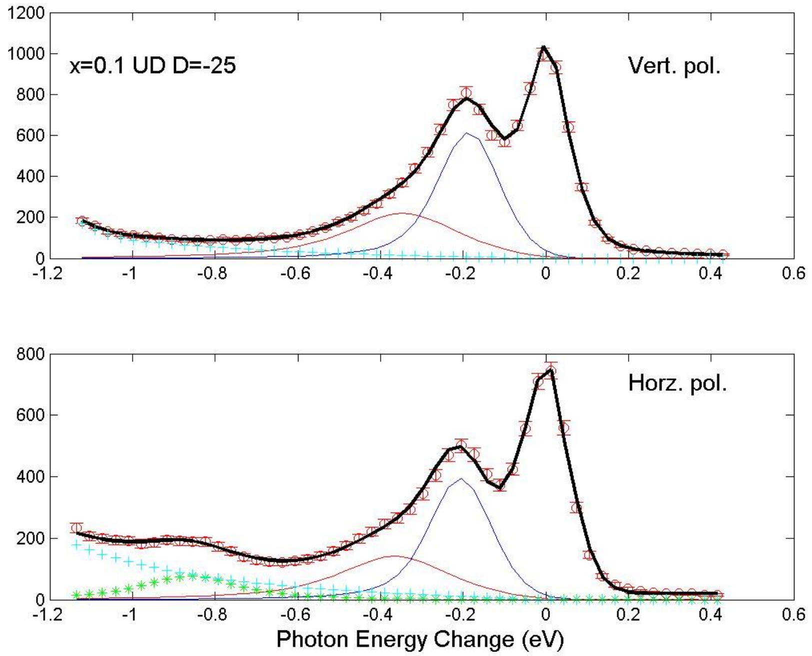
x=0.1 UD D=-25
Vert. pol.
Horz. pol.
Photon Energy Change (eV)

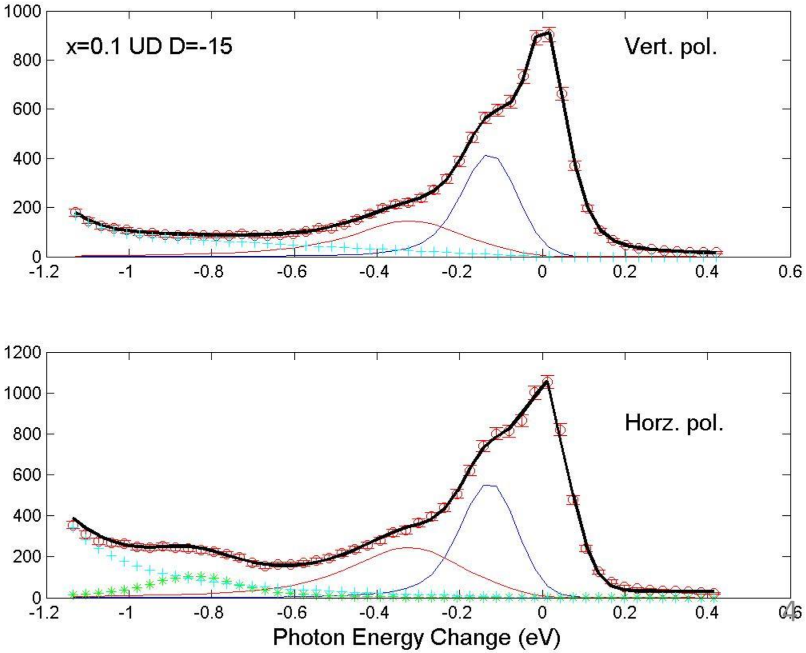
x=0.1 UD D=-15
Vert. pol.
Horz. pol.
Photon Energy Change (eV)

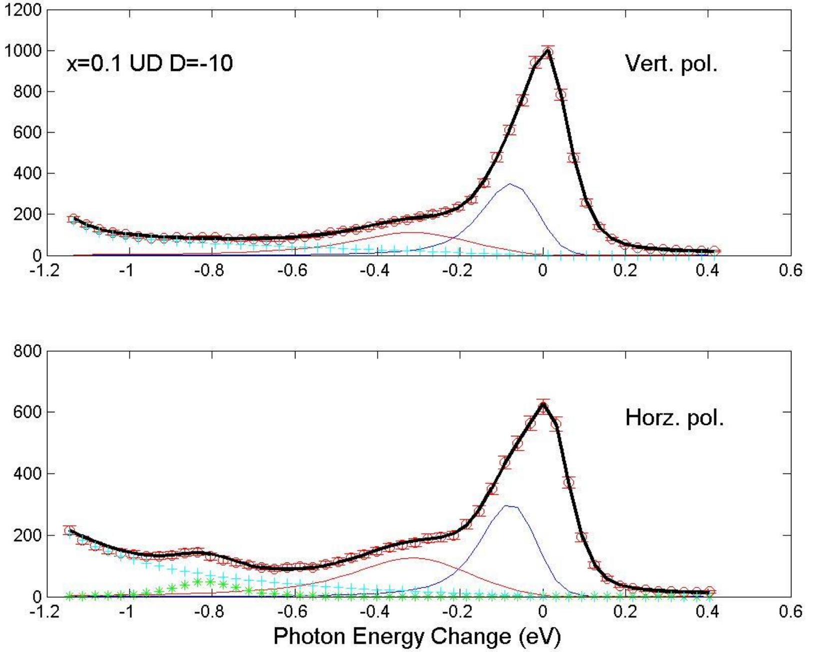
x=0.1 UD D=-10
Vert. pol.
Horz. pol.
Photon Energy Change (eV)

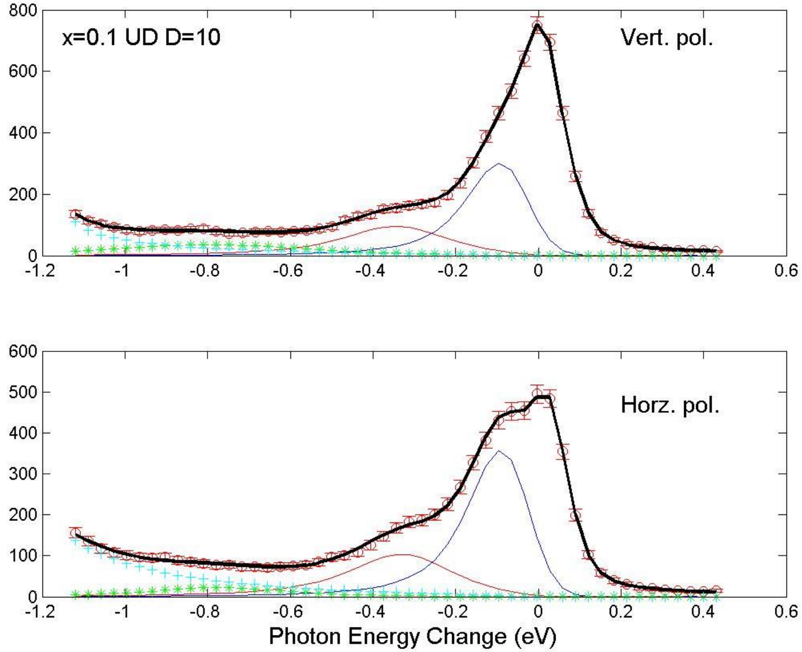
x=0.1 UD D=10
Vert. pol.
Horz. pol.
Photon Energy Change (eV)

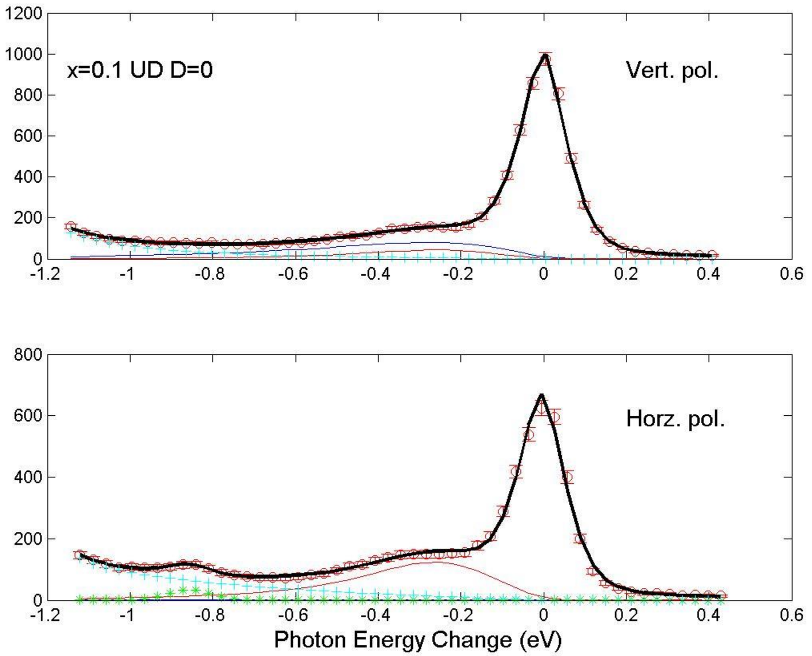
x=0.1 UD D=0
Vert. pol.
Horz. pol.
Photon Energy Change (eV)

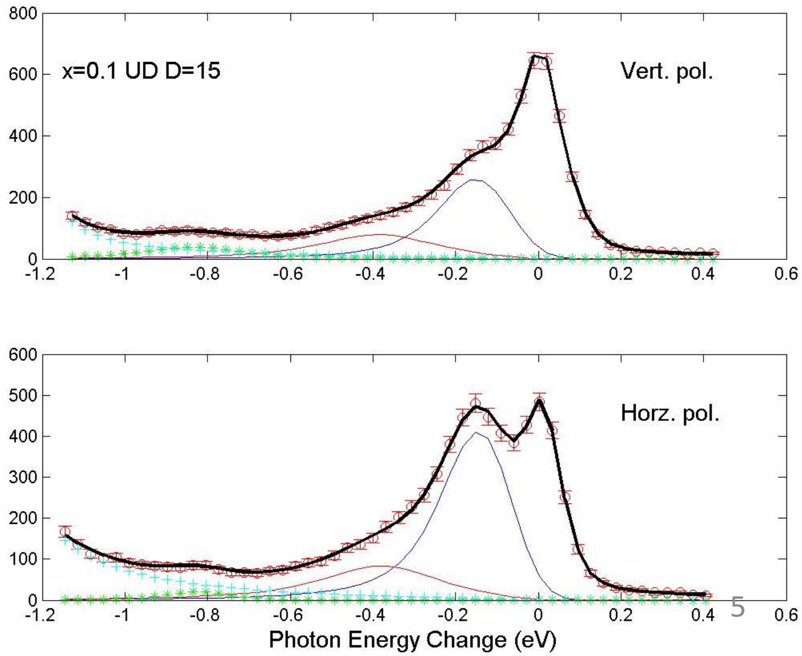
x=0.1 UD D=15
Vert. pol.
Horz. pol.
Photon Energy Change (eV)

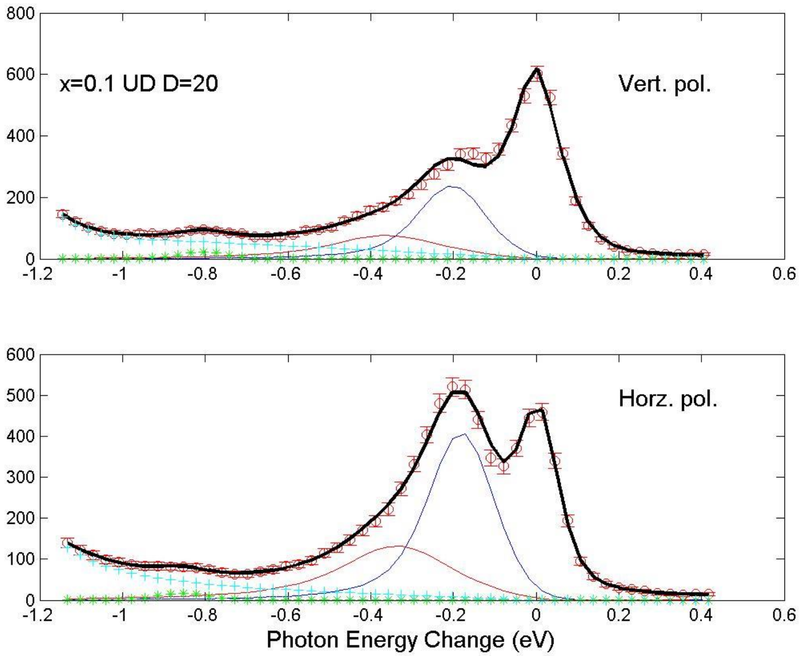
x=0.1 UD D=20
Vert. pol.
Horz. pol.
Photon Energy Change (eV)

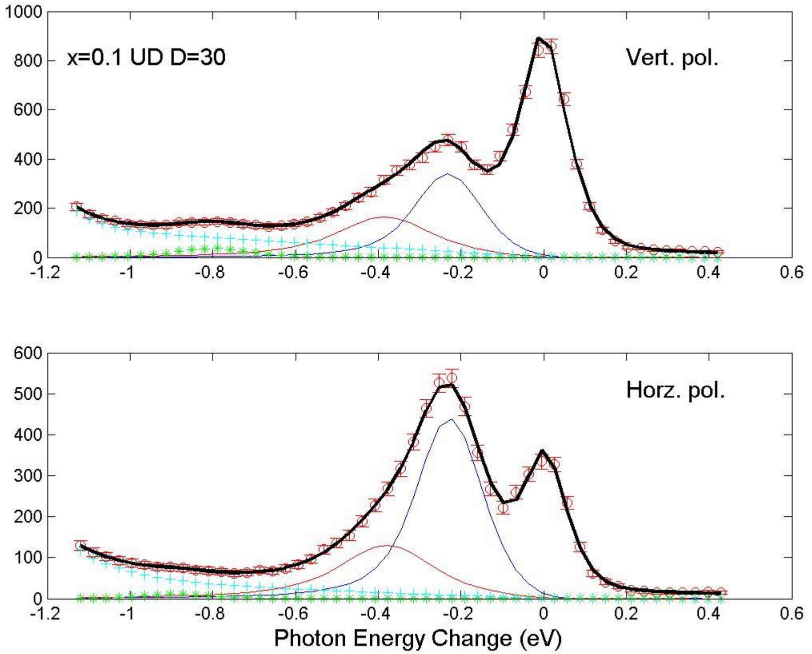
x=0.1 UD D=30
Vert. pol.
Horz. pol.
Photon Energy Change (eV)

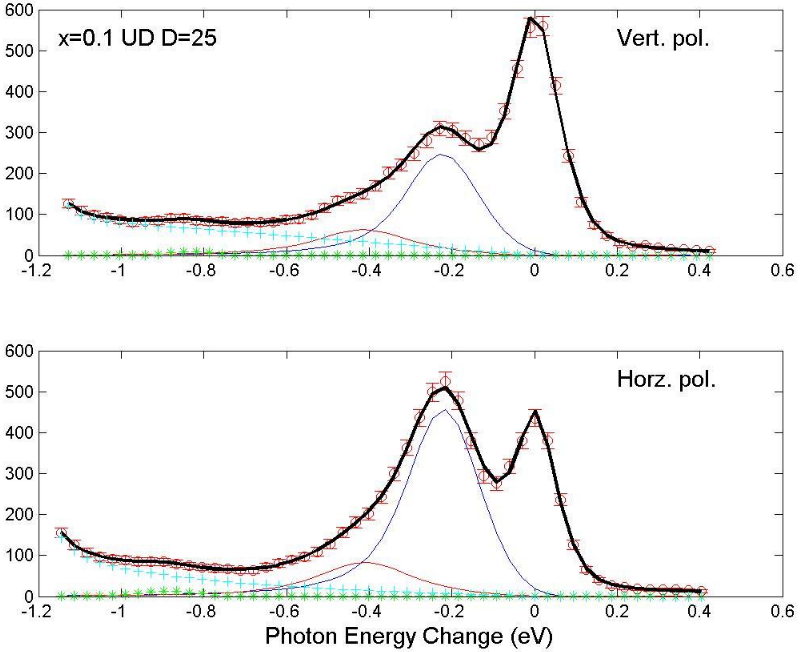
x=0.1 UD D=25
Vert. pol.
Horz. pol.
Photon Energy Change (eV)

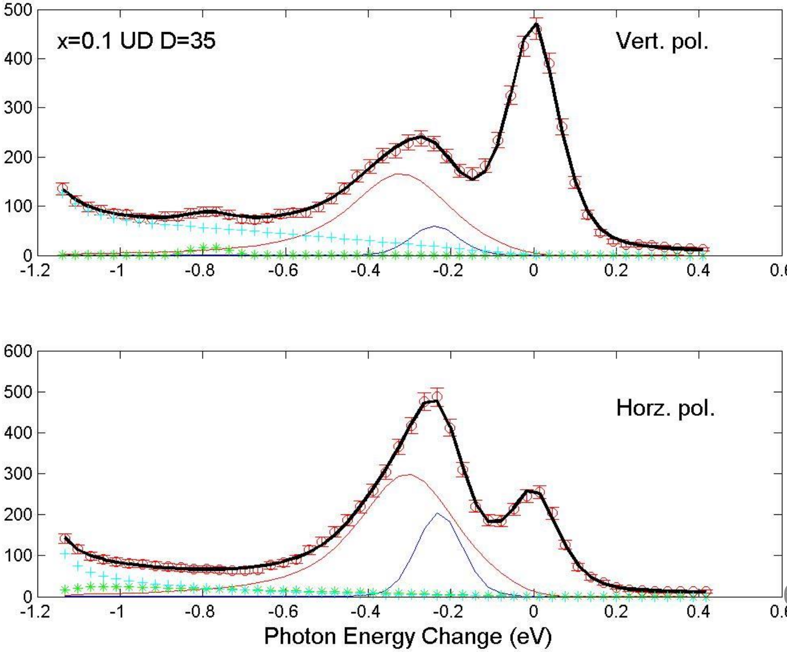
x=0.1 UD D=35
Vert. pol.
Horz. pol.
Photon Energy Change (eV)

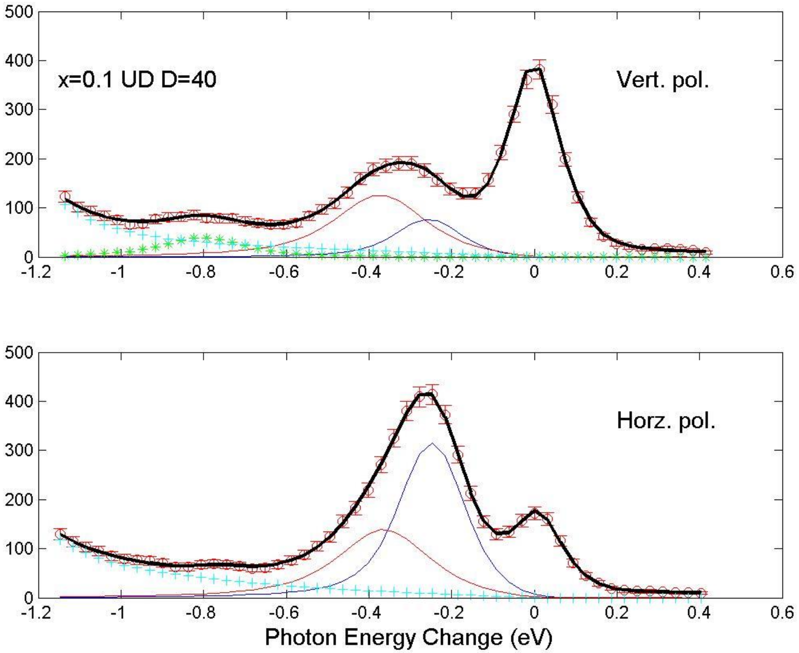
x=0.1 UD D=40
Vert. pol.
Horz. pol.
Photon Energy Change (eV)

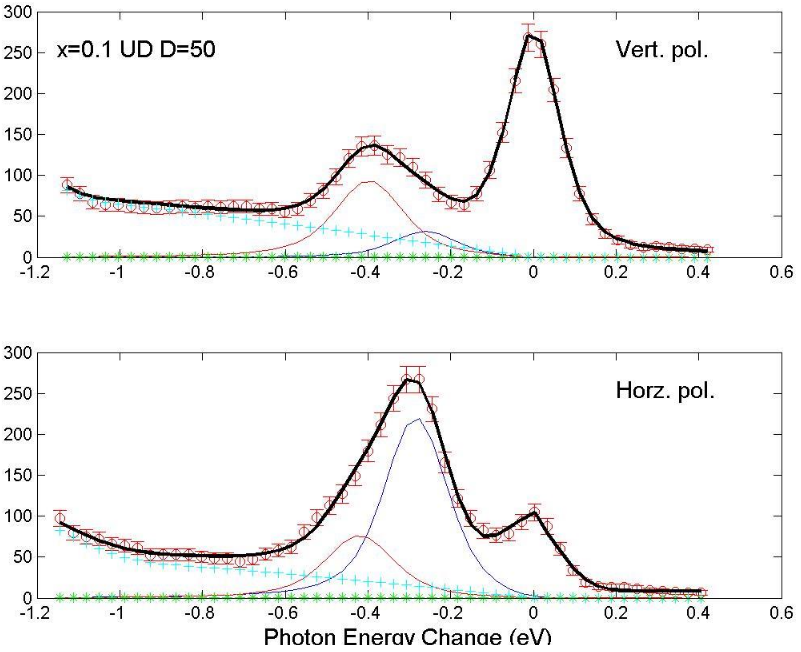
x=0.1 UD D=50
Vert. pol.
Horz. pol.
Photon Energy Change (eV)

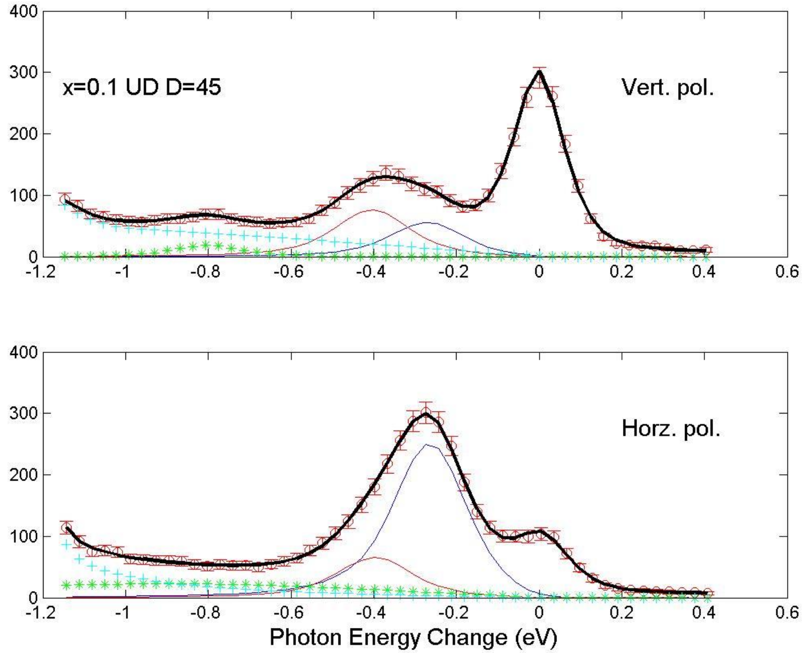
x=0.1 UD D=45
Vert. pol.
Horz. pol.
Photon Energy Change (eV)

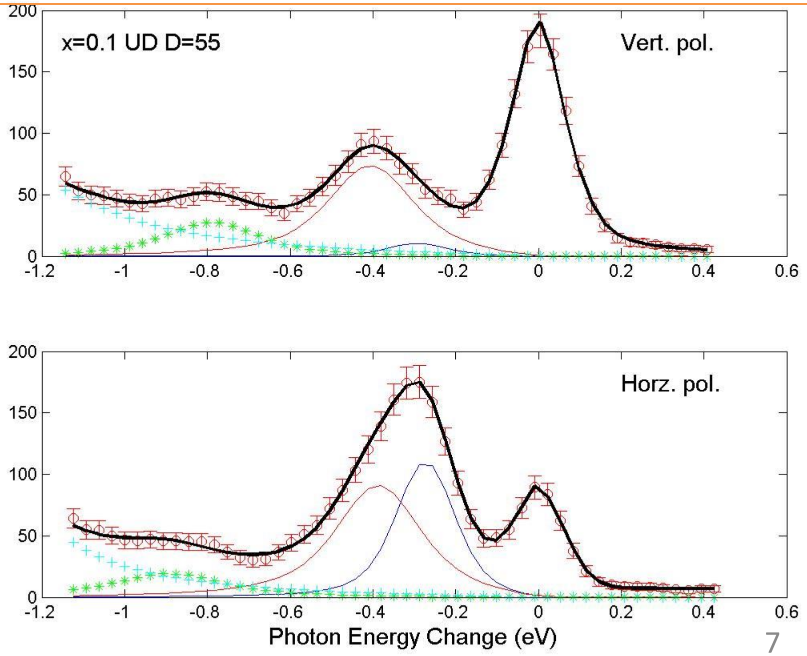
x=0.1 UD D=55
Vert. pol.
Horz. pol.
Photon Energy Change (eV)

x=0.4 under-doped

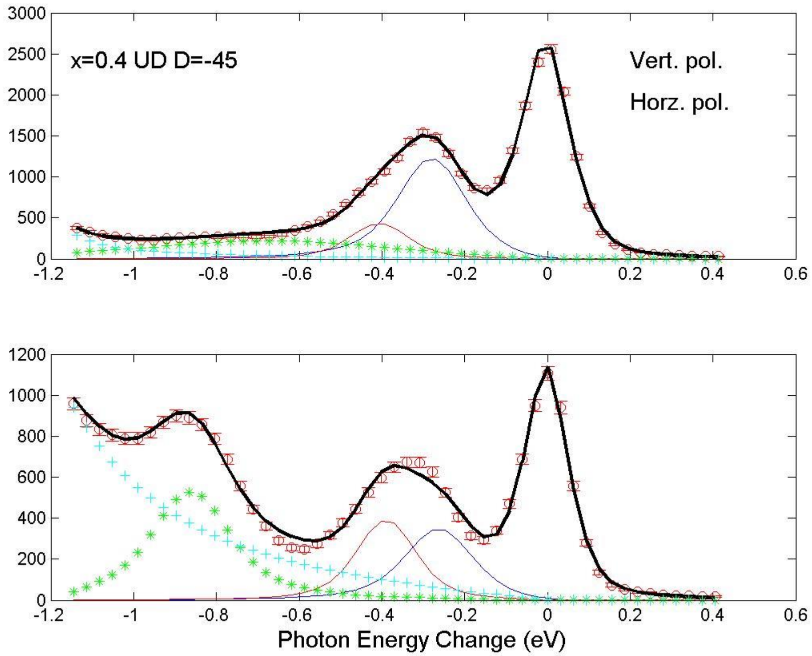


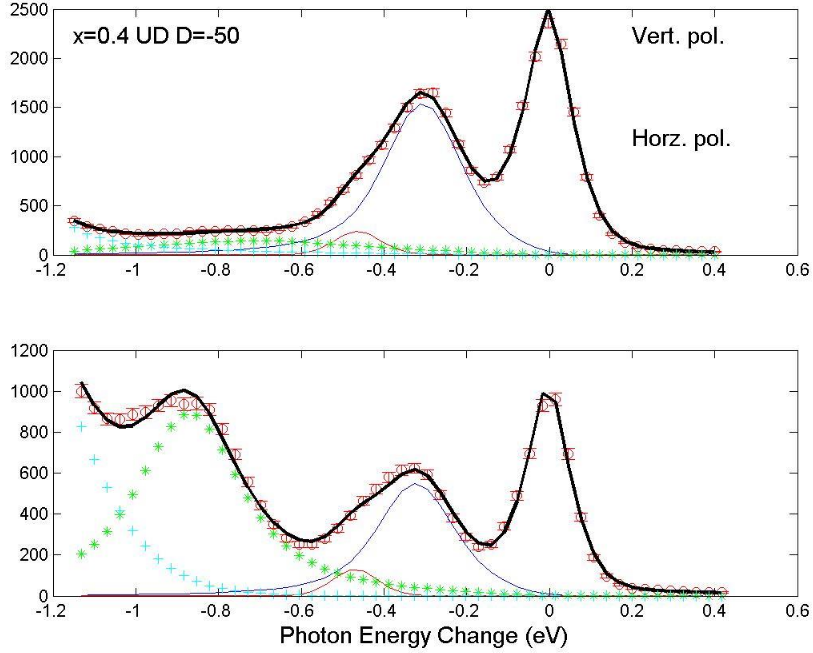


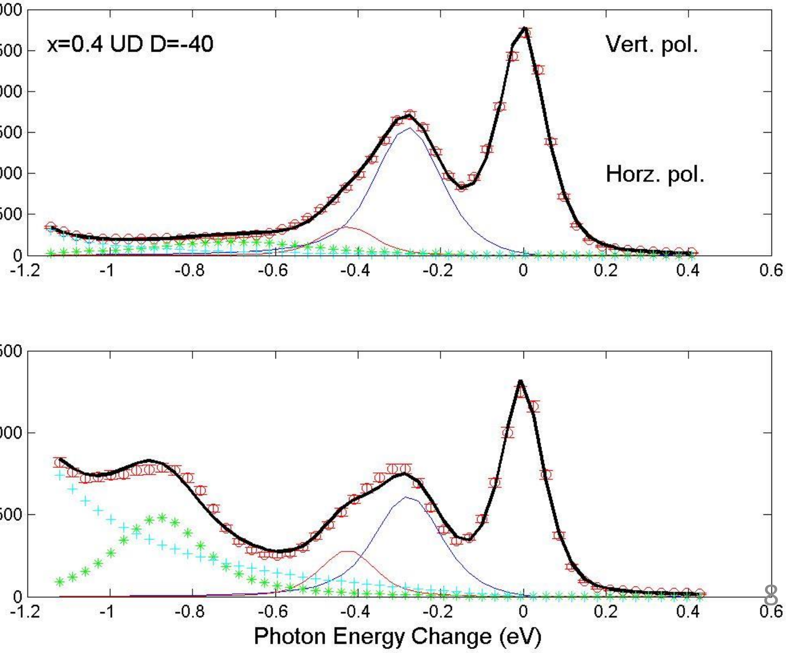

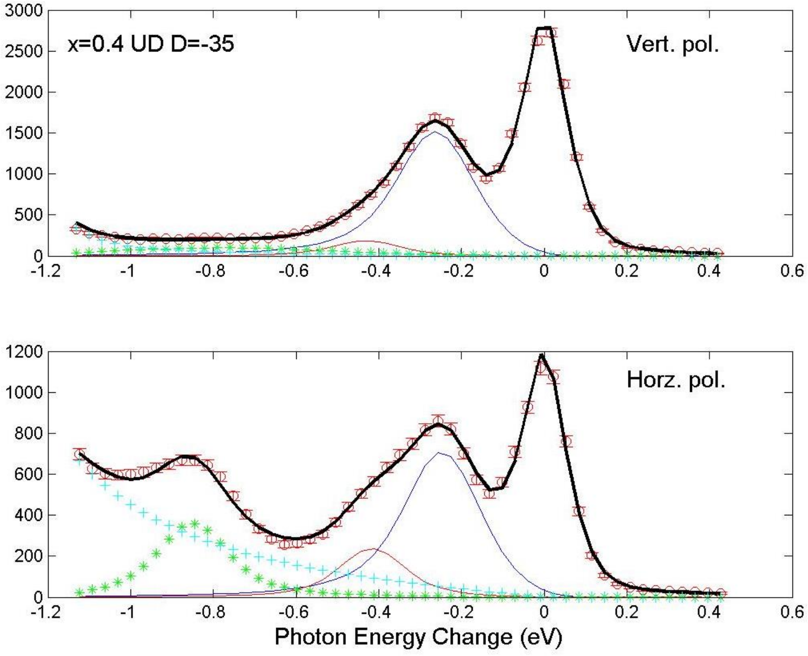
x=0.4 UD D=-35
Vert. pol.
Horz. pol.
Photon Energy Change (eV)

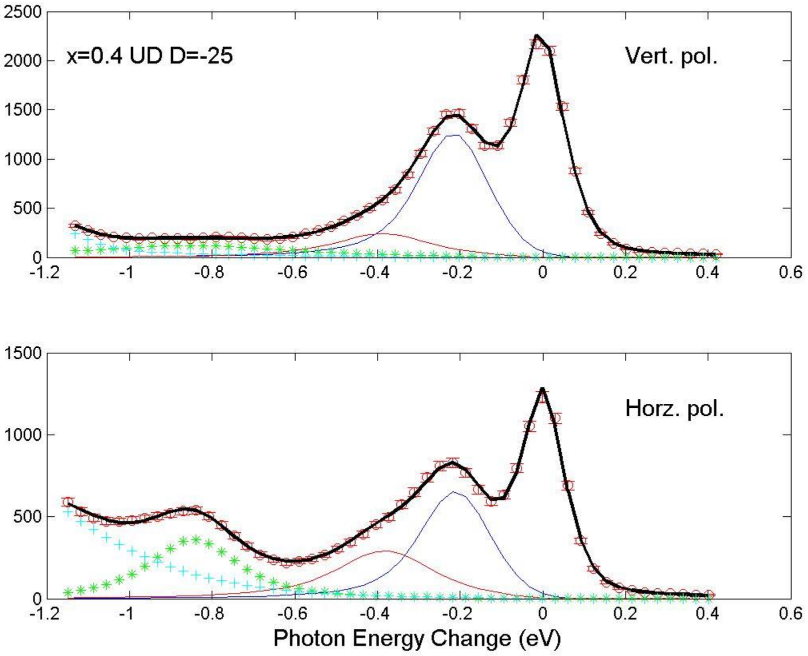
x=0.4 UD D=-25
Vert. pol.
Horz. pol.
Photon Energy Change (eV)

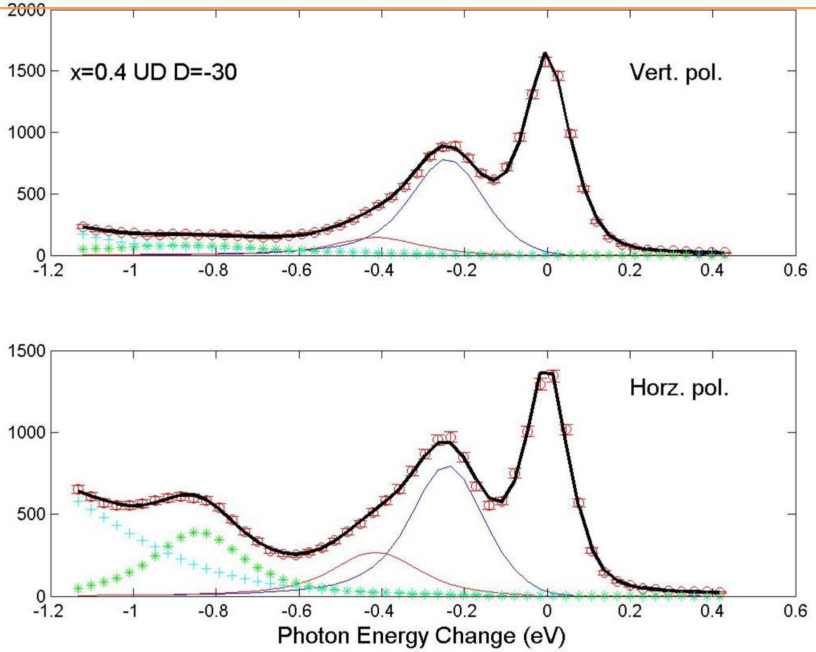
x=0.4 UD D=-30
Vert. pol.
Horz. pol.
Photon Energy Change (eV)

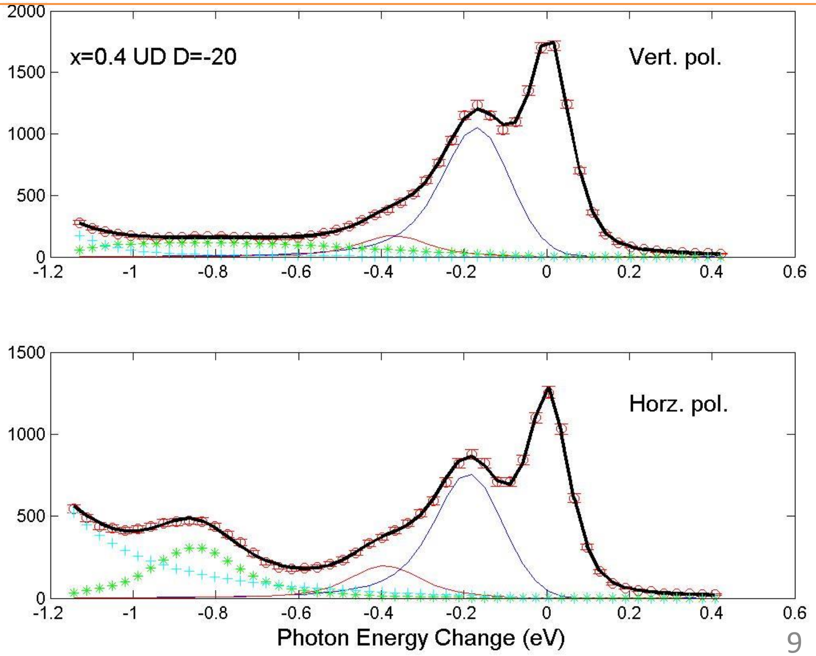
x=0.4 UD D=-20
Vert. pol.
Horz. pol.
Photon Energy Change (eV)

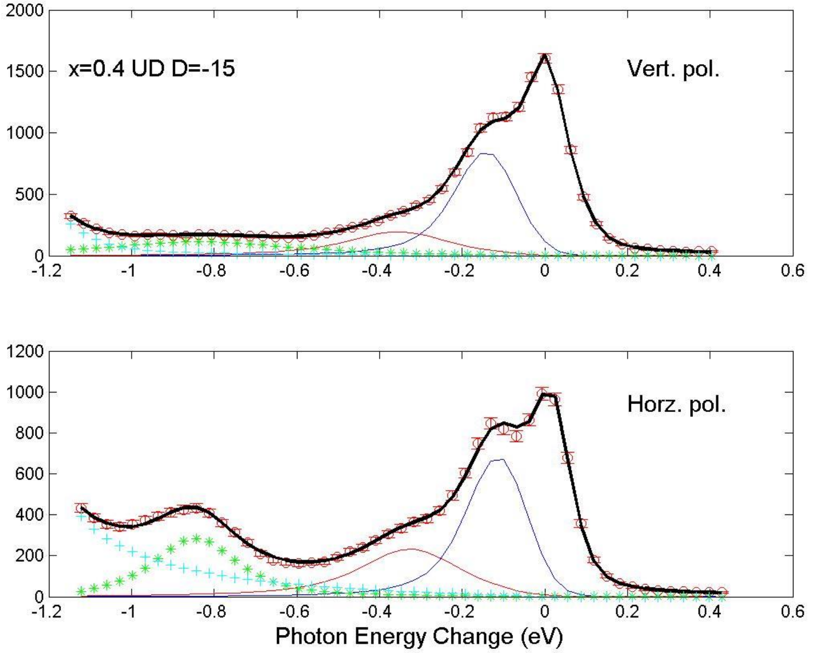
x=0.4 UD D=-15
Vert. pol.
Horz. pol.
Photon Energy Change (eV)

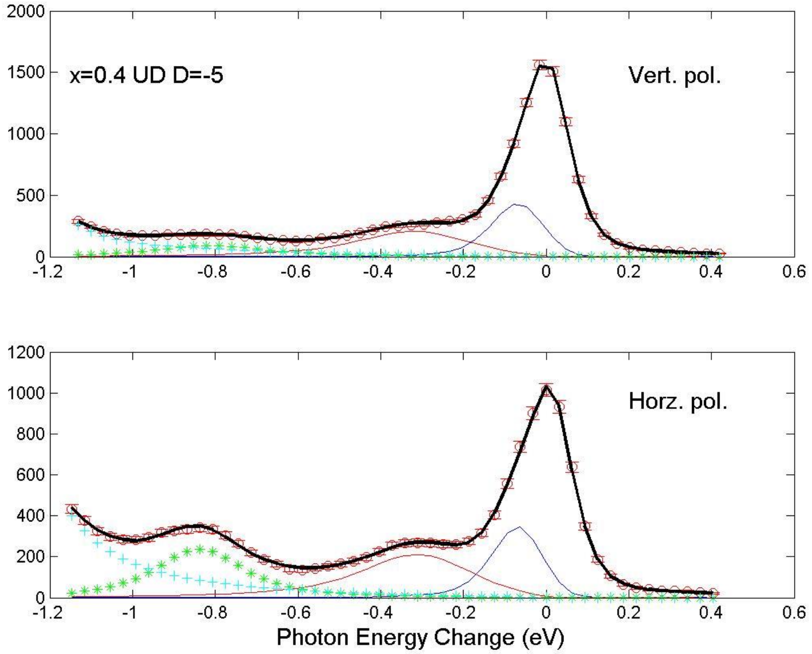
x=0.4 UD D=-5
Vert. pol.
Horz. pol.
Photon Energy Change (eV)

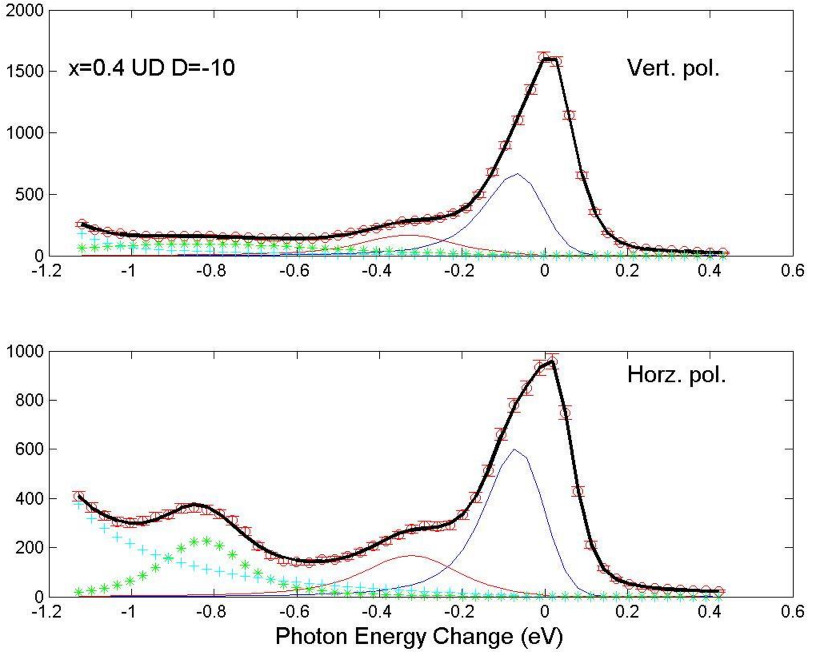
x=0.4 UD D=-10
Vert. pol.
Horz. pol.
Photon Energy Change (eV)

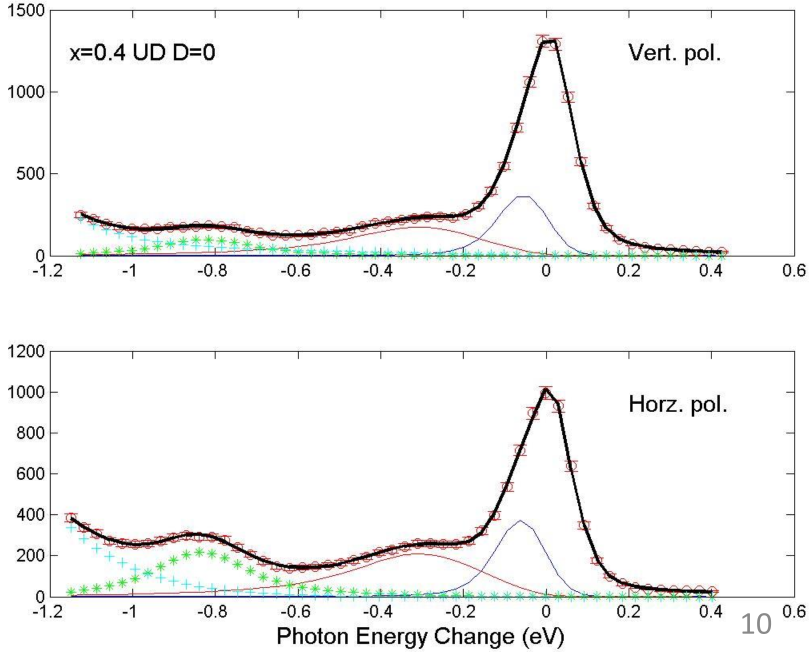
x=0.4 UD D=0
Vert. pol.
Horz. pol.
Photon Energy Change (eV)

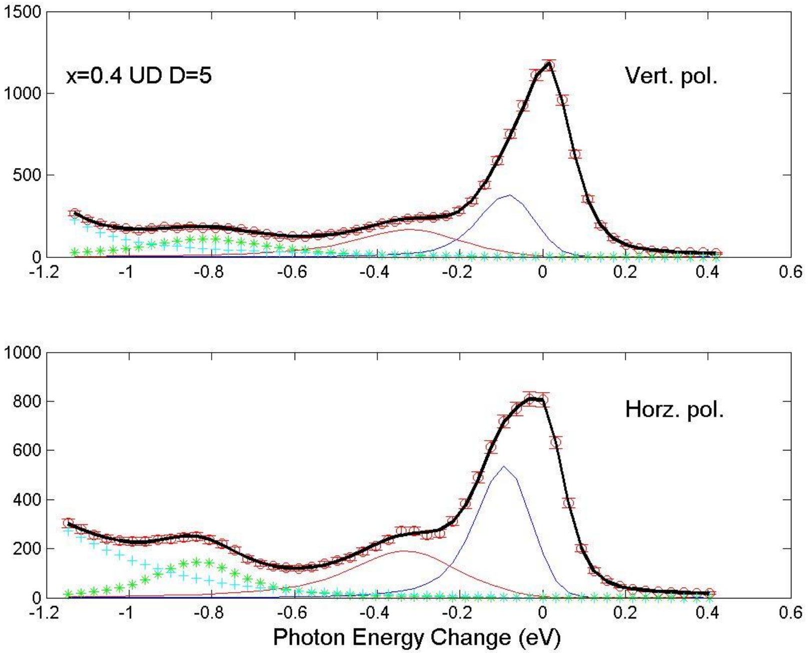
x=0.4 UD D=5
Vert. pol.
Horz. pol.
Photon Energy Change (eV)

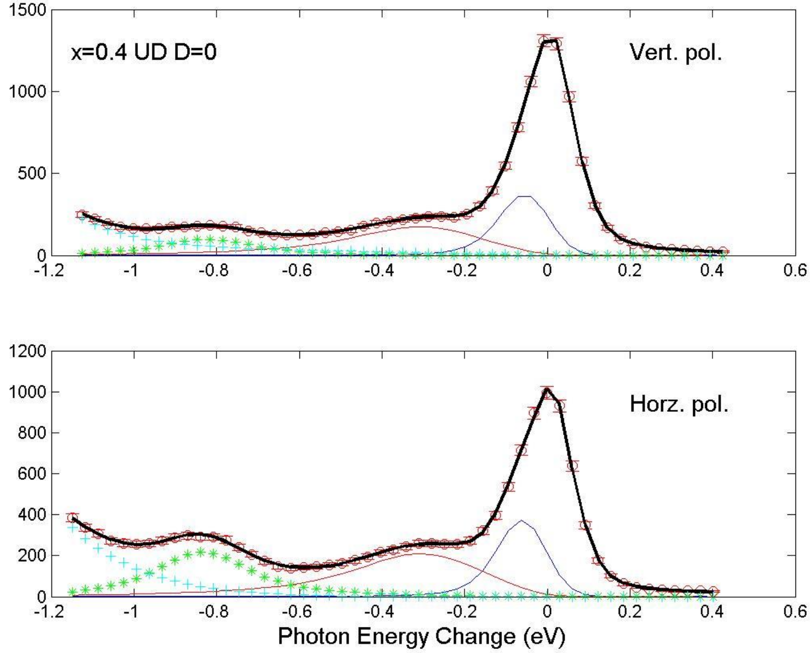
x=0.4 UD D=0
Vert. pol.
Horz. pol.
Photon Energy Change (eV)

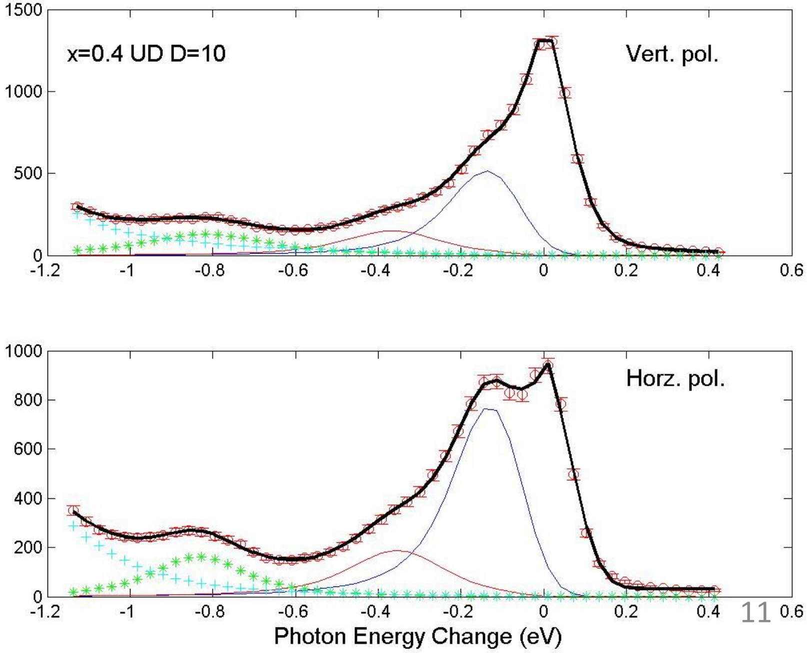
x=0.4 UD D=10
Vert. pol.
Horz. pol.
Photon Energy Change (eV)

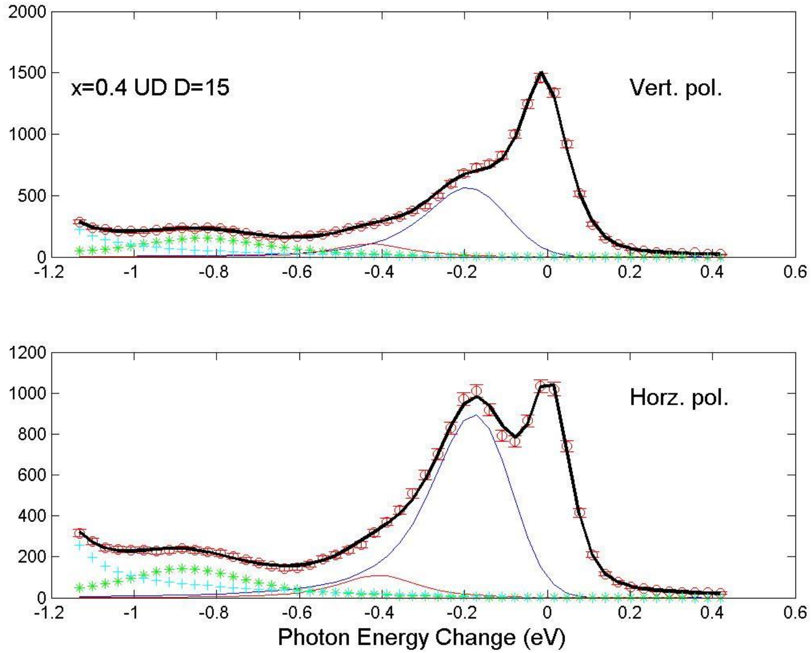
x=0.4 UD D=15
Vert. pol.
Horz. pol.
Photon Energy Change (eV)

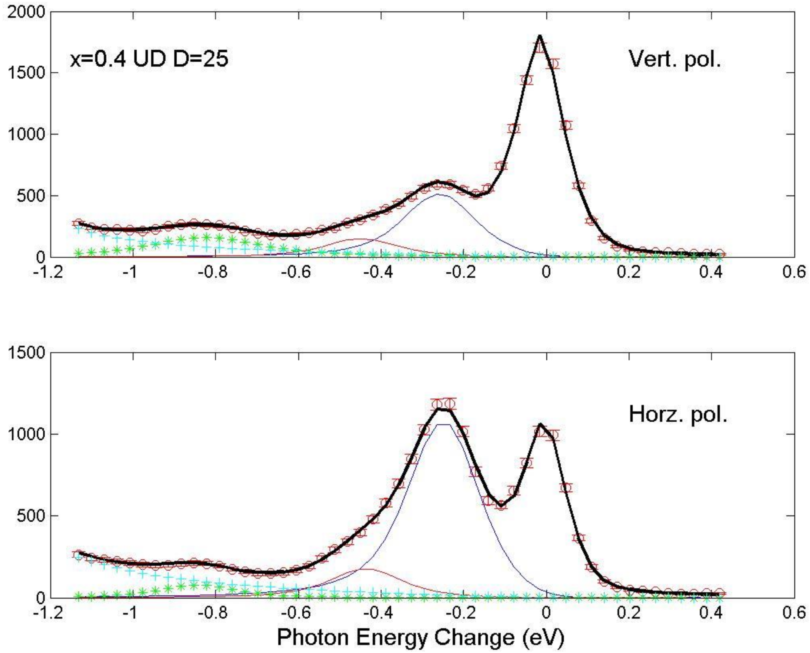
x=0.4 UD D=25
Vert. pol.
Horz. pol.
Photon Energy Change (eV)

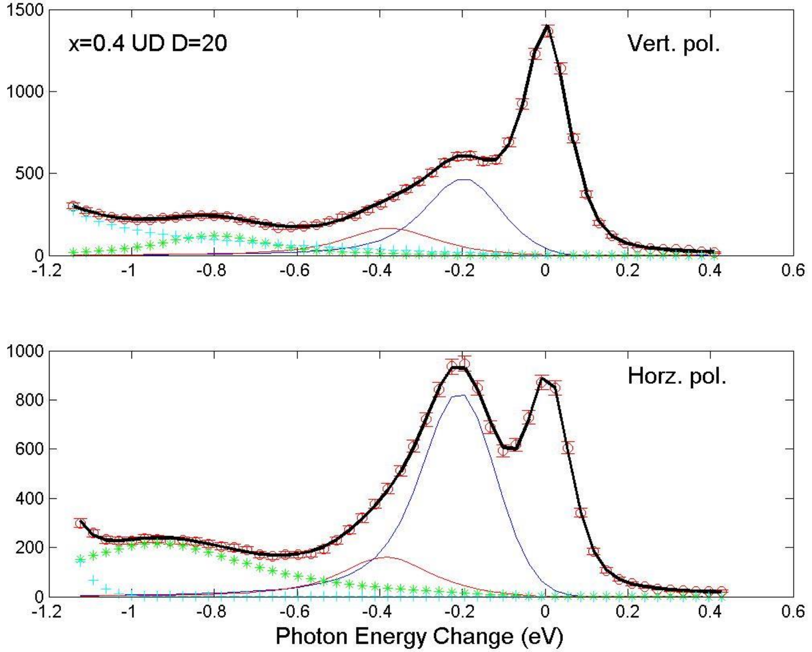
x=0.4 UD D=20
Vert. pol.
Horz. pol.
Photon Energy Change (eV)

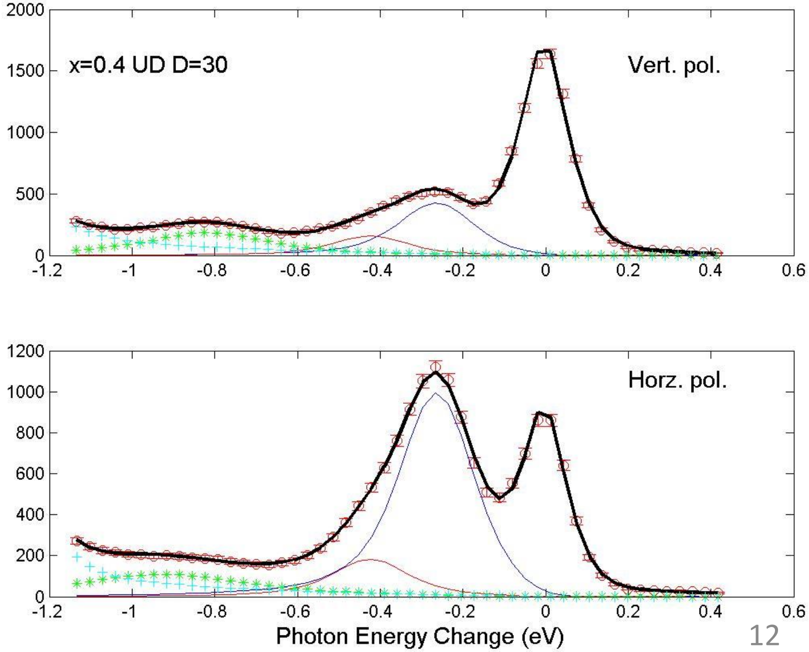
x=0.4 UD D=30
Vert. pol.
Horz. pol.
Photon Energy Change (eV)

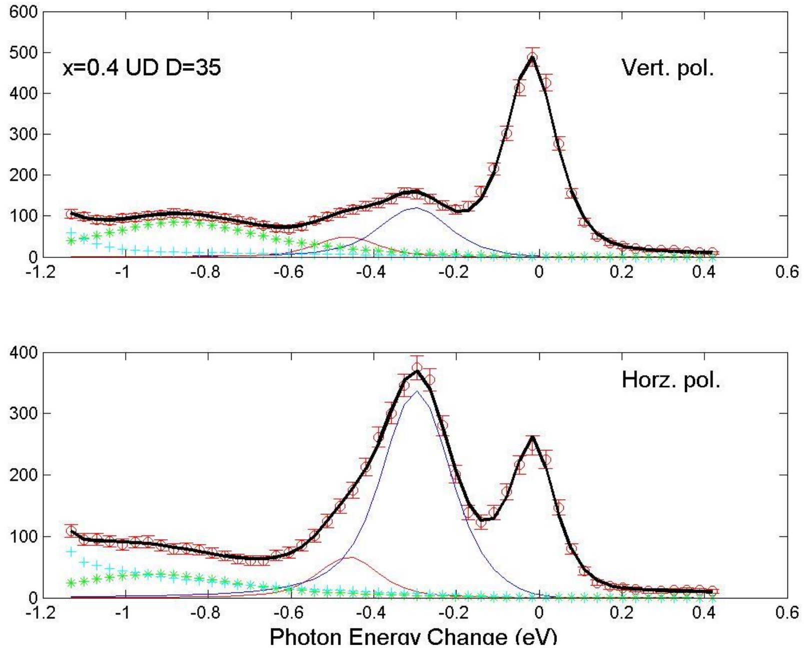
x=0.4 UD D=35
Vert. pol.
Horz. pol.
Photon Energy Change (eV)

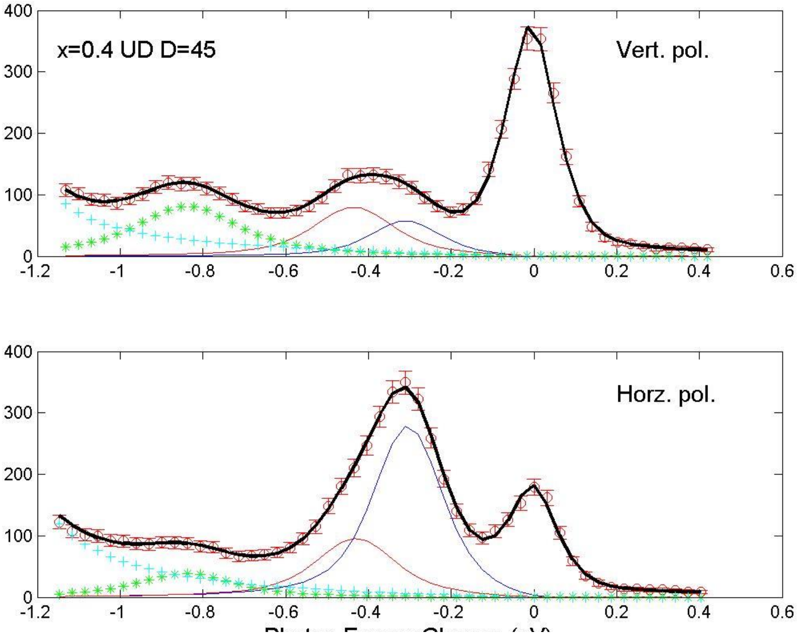
x=0.4 UD D=45
Vert. pol.
Horz. pol.

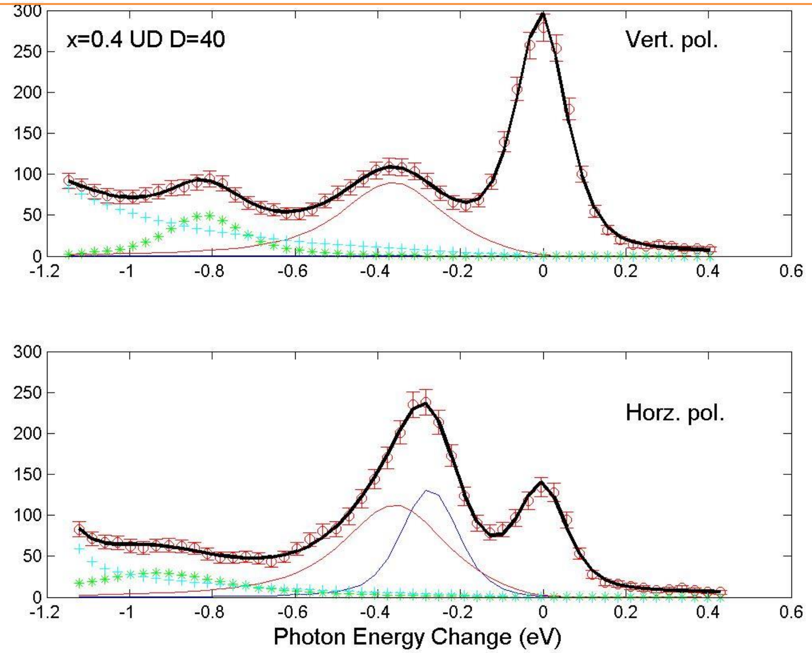
x=0.4 UD D=40
Vert. pol.
Horz. pol.
Photon Energy Change (eV)

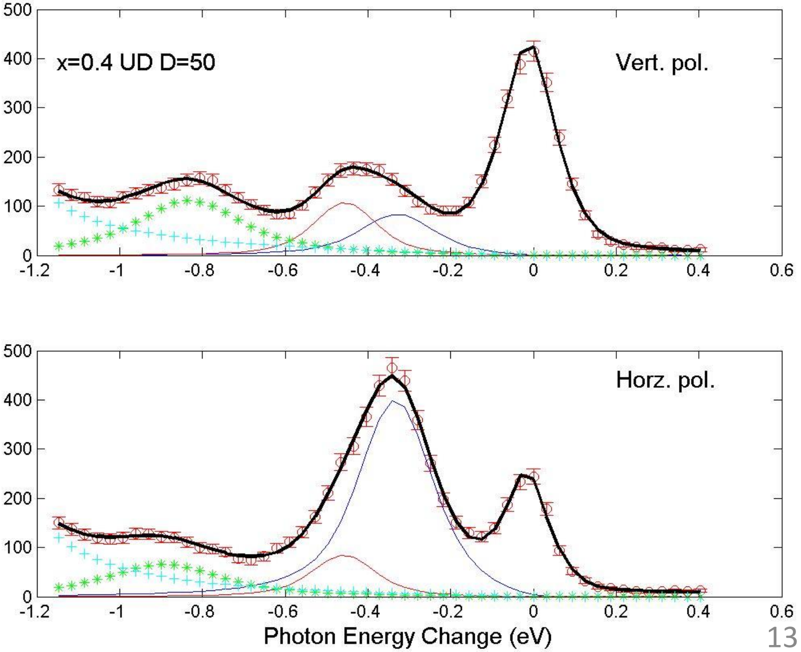
x=0.4 UD D=50
Vert. pol.
Horz. pol.
Photon Energy Change (eV)

## 2. Optimally Doped Samples : Paramagnon Fits

These were done using a single magnetic component in place of the 1-magnon+2-magnon used for UD, as described in the main text. Only the π- (horizontally) polarized spectra were used. Nine *D*-positions per page are shown, with the raw data, total fit, and asymmetric fit for the magnetic component displayed. The resultant energy, width and intensity fit parameters for this peak are indicated on each graph.

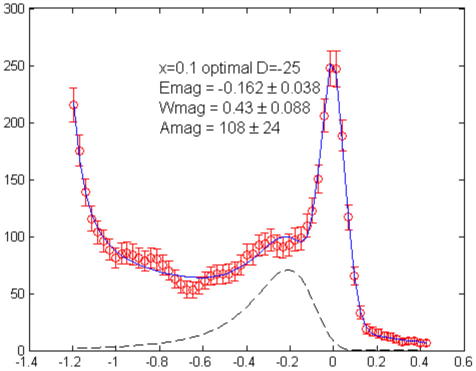
x=0.1 optimal D=-25
Emag = -0.162 ± 0.038
Wmag = 0.43 ± 0.088
Amag = 108 ± 24

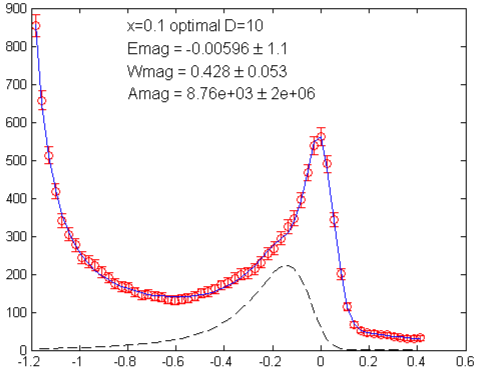
x=0.1 optimal D=10
Emag = -0.00596 ± 1.1
Wmag = 0.428 ± 0.053
Amag = 8.76e+03 ± 2e+06

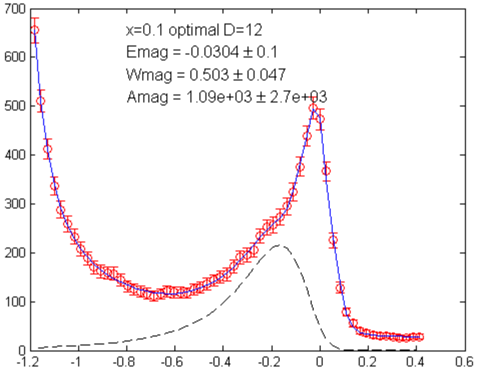
x=0.1 optimal D=12
Emag = -0.0304 ± 0.1
Wmag = 0.503 ± 0.047
Amag = 1.09e+03 ± 2.7e+03

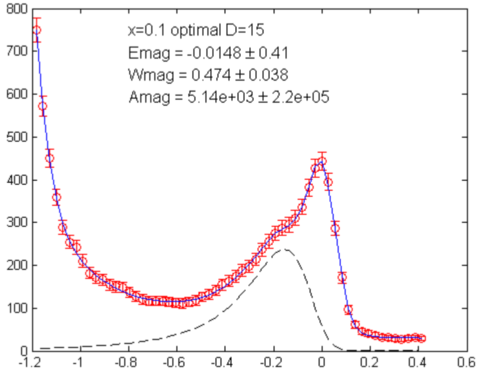
x=0.1 optimal D=15
Emag = -0.0148 ± 0.41
Wmag = 0.474 ± 0.038
Amag = 5.14e+03 ± 2.2e+05

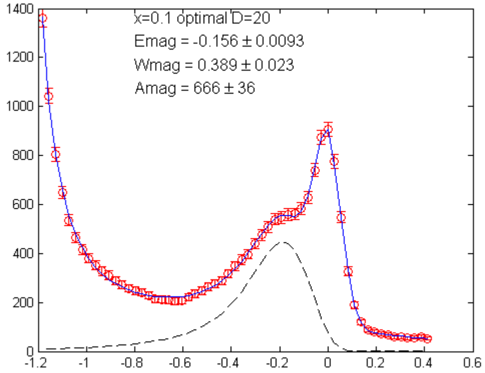
x=0.1 optimal D=20
Emag = -0.156 ± 0.0093
Wmag = 0.389 ± 0.023
Amag = 666 ± 36

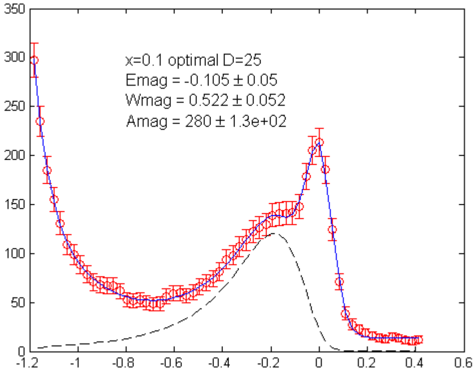
x=0.1 optimal D=25
Emag = -0.105 ± 0.05
Wmag = 0.522 ± 0.052
Amag = 280 ± 1.3e+02

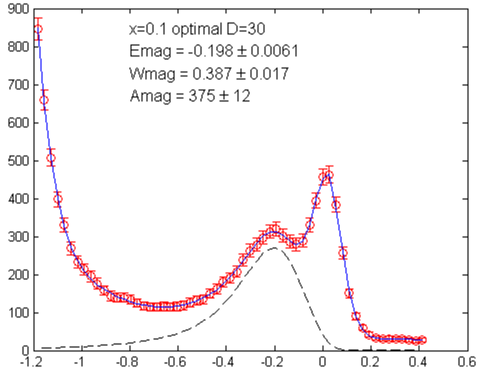
x=0.1 optimal D=30
Emag = -0.198 ± 0.0061
Wmag = 0.387 ± 0.017
Amag = 375 ± 12

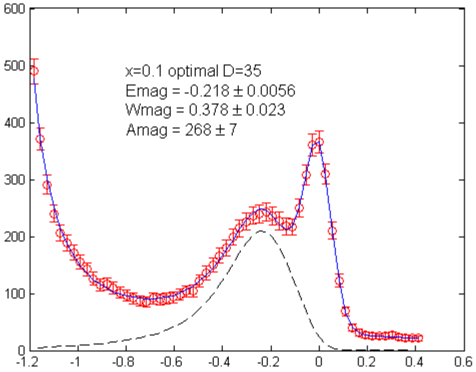
x=0.1 optimal D=35
Emag = -0.218 ± 0.0056
Wmag = 0.378 ± 0.023
Amag = 268 ± 7

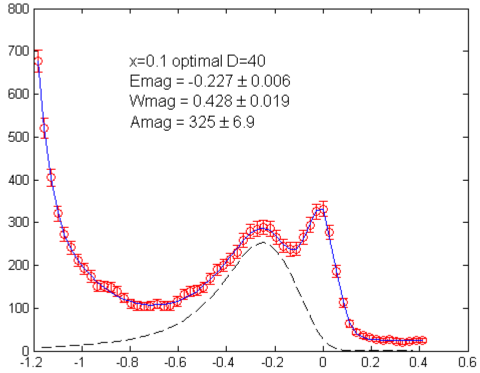
x=0.1 optimal D=40
Emag = -0.227 ± 0.006
Wmag = 0.428 ± 0.019
Amag = 325 ± 6.9

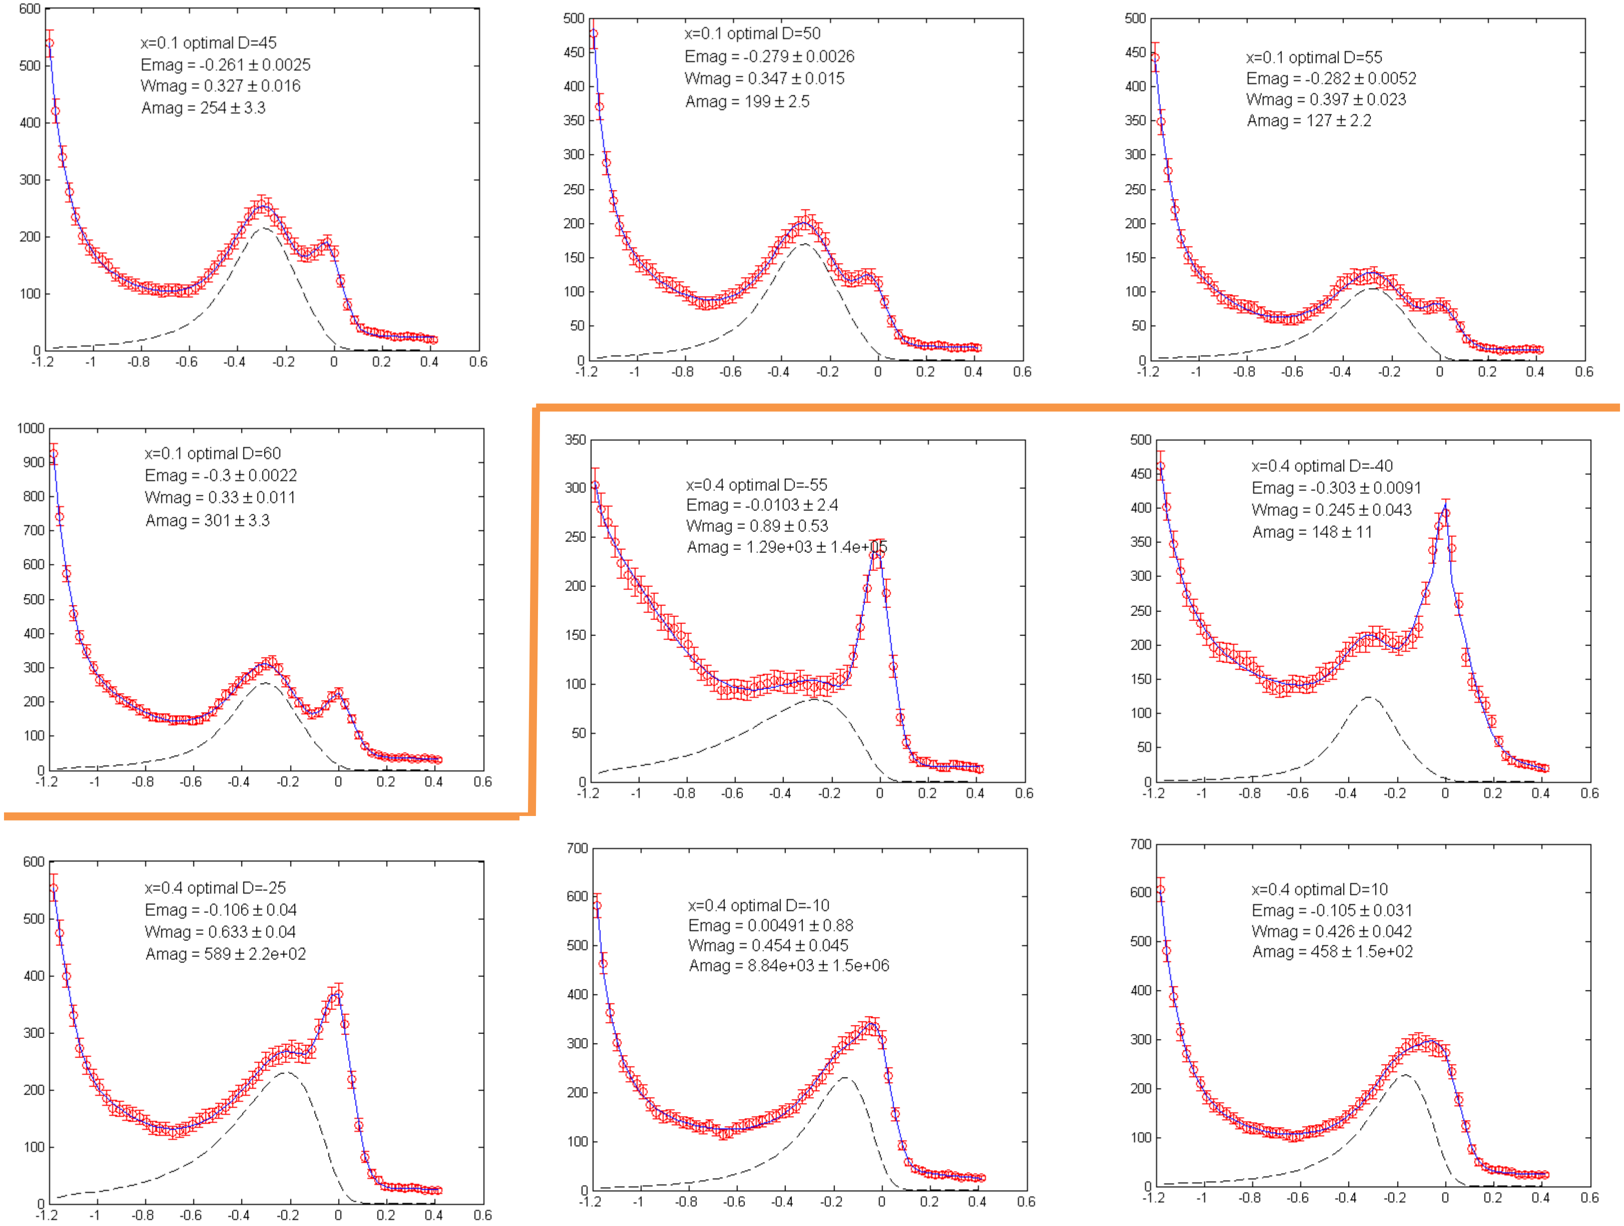

x=0.1 optimal D=45
Emag = -0.261 ± 0.0025
Wmag = 0.327 ± 0.016
Amag = 254 ± 3.3
x=0.1 optimal D=50
Emag = -0.279 ± 0.0026
Wmag = 0.347 ± 0.015
Amag = 199 ± 2.5
x=0.1 optimal D=55
Emag = -0.282 ± 0.0052
Wmag = 0.397 ± 0.023
Amag = 127 ± 2.2
x=0.1 optimal D=60
Emag = -0.3 ± 0.0022
Wmag = 0.33 ± 0.011
Amag = 301 ± 3.3
x=0.4 optimal D=-55
Emag = -0.0103 ± 2.4
Wmag = 0.89 ± 0.53
Amag = 1.29e+03 ± 1.4e+05
x=0.4 optimal D=-40
Emag = -0.303 ± 0.0091
Wmag = 0.245 ± 0.043
Amag = 148 ± 11
x=0.4 optimal D=-25
Emag = -0.106 ± 0.04
Wmag = 0.633 ± 0.04
Amag = 589 ± 2.2e+02
x=0.4 optimal D=-10
Emag = 0.00491 ± 0.88
Wmag = 0.454 ± 0.045
Amag = 8.84e+03 ± 1.5e+06
x=0.4 optimal D=10
Emag = -0.105 ± 0.031
Wmag = 0.426 ± 0.042
Amag = 458 ± 1.5e+02

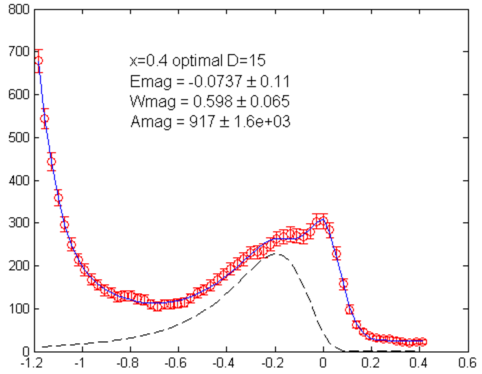
x=0.4 optimal D=15
Emag = -0.0737 ± 0.11
Wmag = 0.598 ± 0.065
Amag = 917 ± 1.6e+03

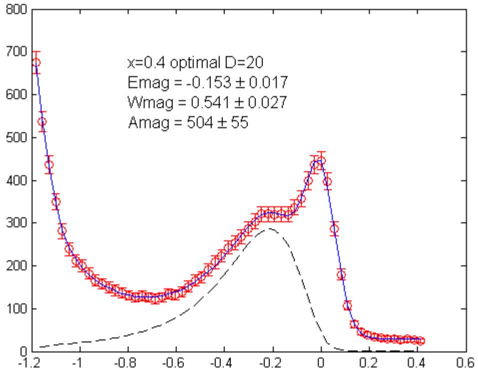
x=0.4 optimal D=20
Emag = -0.153 ± 0.017
Wmag = 0.541 ± 0.027
Amag = 504 ± 55

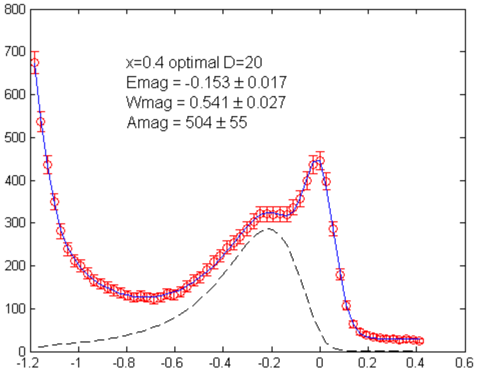
x=0.4 optimal D=20
Emag = -0.153 ± 0.017
Wmag = 0.541 ± 0.027
Amag = 504 ± 55

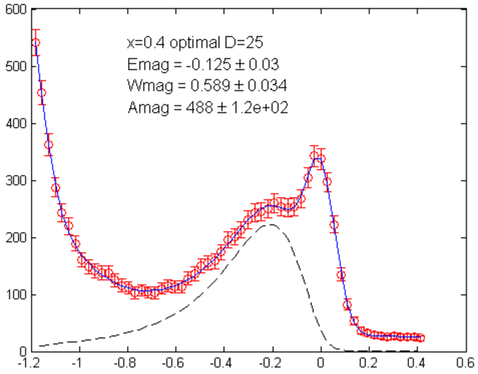
x=0.4 optimal D=25
Emag = -0.125 ± 0.03
Wmag = 0.589 ± 0.034
Amag = 488 ± 1.2e+02

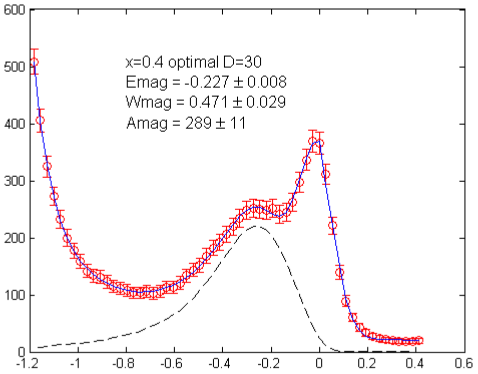
x=0.4 optimal D=30
Emag = -0.227 ± 0.008
Wmag = 0.471 ± 0.029
Amag = 289 ± 11

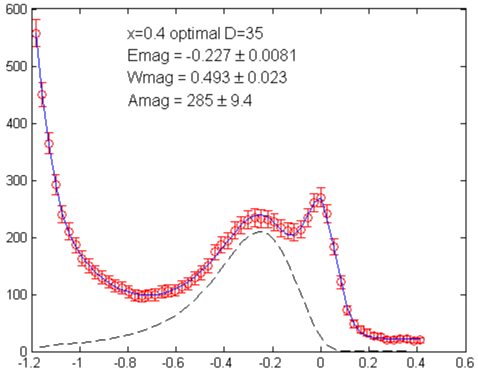
x=0.4 optimal D=35
Emag = -0.227 ± 0.0081
Wmag = 0.493 ± 0.023
Amag = 285 ± 9.4

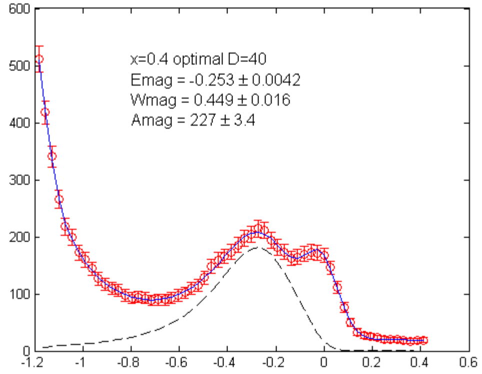
x=0.4 optimal D=40
Emag = -0.253 ± 0.0042
Wmag = 0.449 ± 0.016
Amag = 227 ± 3.4

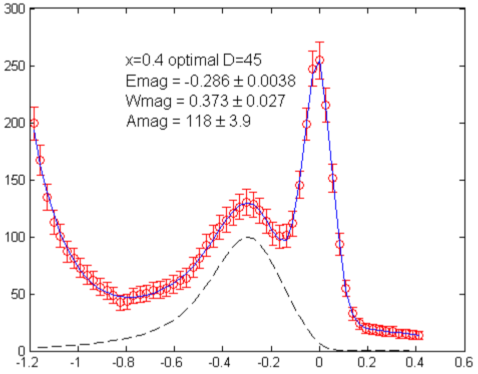
x=0.4 optimal D=45
Emag = -0.286 ± 0.0038
Wmag = 0.373 ± 0.027
Amag = 118 ± 3.9

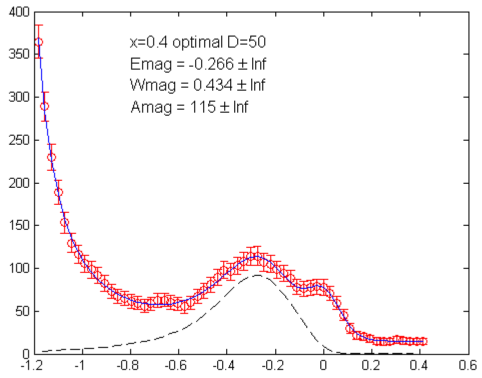
x=0.4 optimal D=50
Emag = -0.266 ± Inf
Wmag = 0.434 ± Inf
Amag = 115 ± Inf

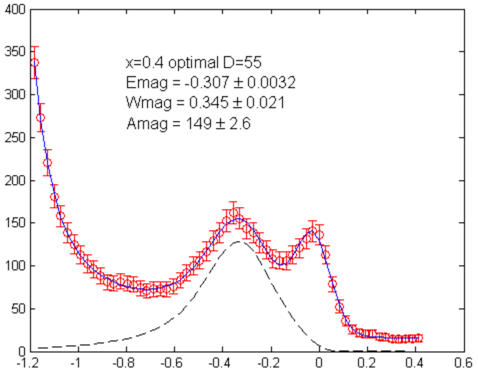
x=0.4 optimal D=55
Emag = -0.307 ± 0.0032
Wmag = 0.345 ± 0.021
Amag = 149 ± 2.6

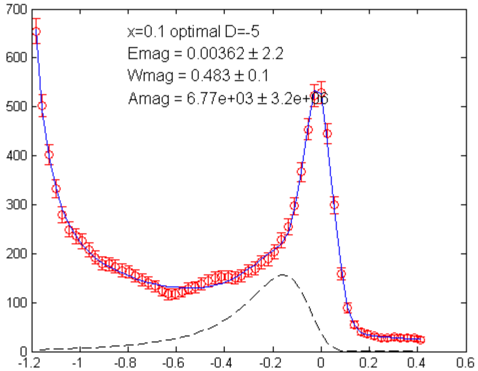
x=0.1 optimal D=-5
Emag = 0.00362 ± 2.2
Wmag = 0.483 ± 0.1

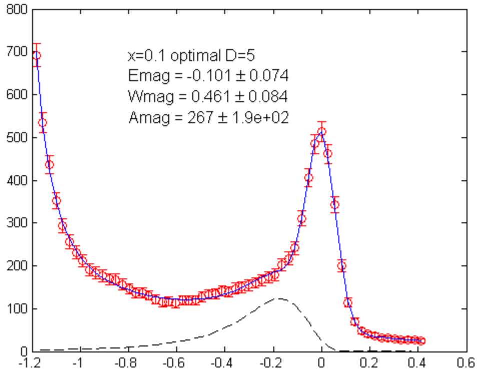
x=0.1 optimal D=5
Emag = -0.101 ± 0.074
Wmag = 0.461 ± 0.084
Amag = 267 ± 1.9e+02

# Undoped Samples : *dd* excitation fits

The *dd* excitation fits to 3 Gaussians+constant, sharing energy and width parameters for horizontal and vertical polarizations, as described in the main text. The initial parameters were the same for all fits. The intensities here are normalized by the high-energy (10-13 eV) part of RIXS spectra. The fitting was done over the range as shown on the graphs. To rule out that the very small dispersions observed are not due to center energy being off in systematic way, we checked that the elastic lines of all the spectra are centered, as shown in the graphs below.

Centering of quasi-elastic peaks:

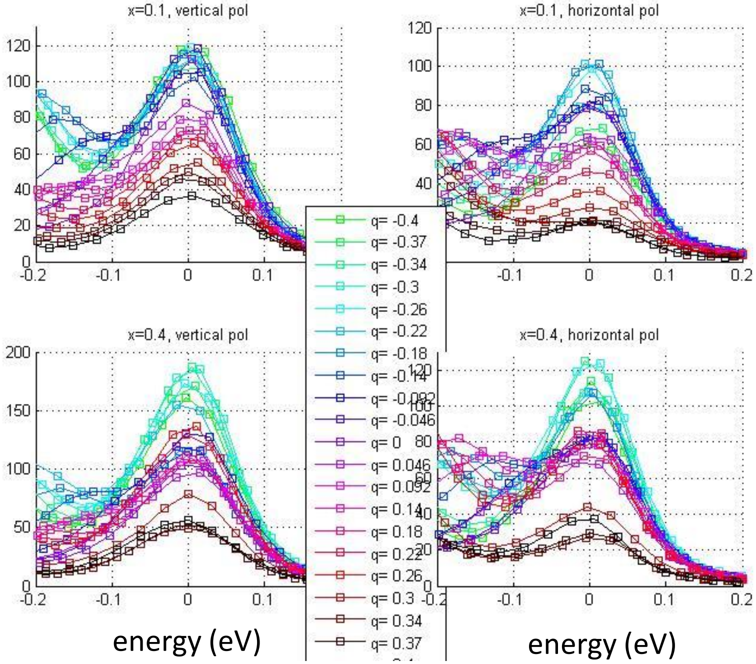


In 3 places fitting was slightly skewed. It seems like there may be a mild peak at 2.3 eV, seen for horizontal polarization, near extreme negative *D*. This was observed for both *x*=0.1 and *x*=0.4, at *D*=-50, and *x*=0.4 at *D*=-40.

Page Layout for Following Pages of Fits (4 q's per page)
(-Delta ("D") on left, + on right, Vertical polarization on top, Horz on bottom :

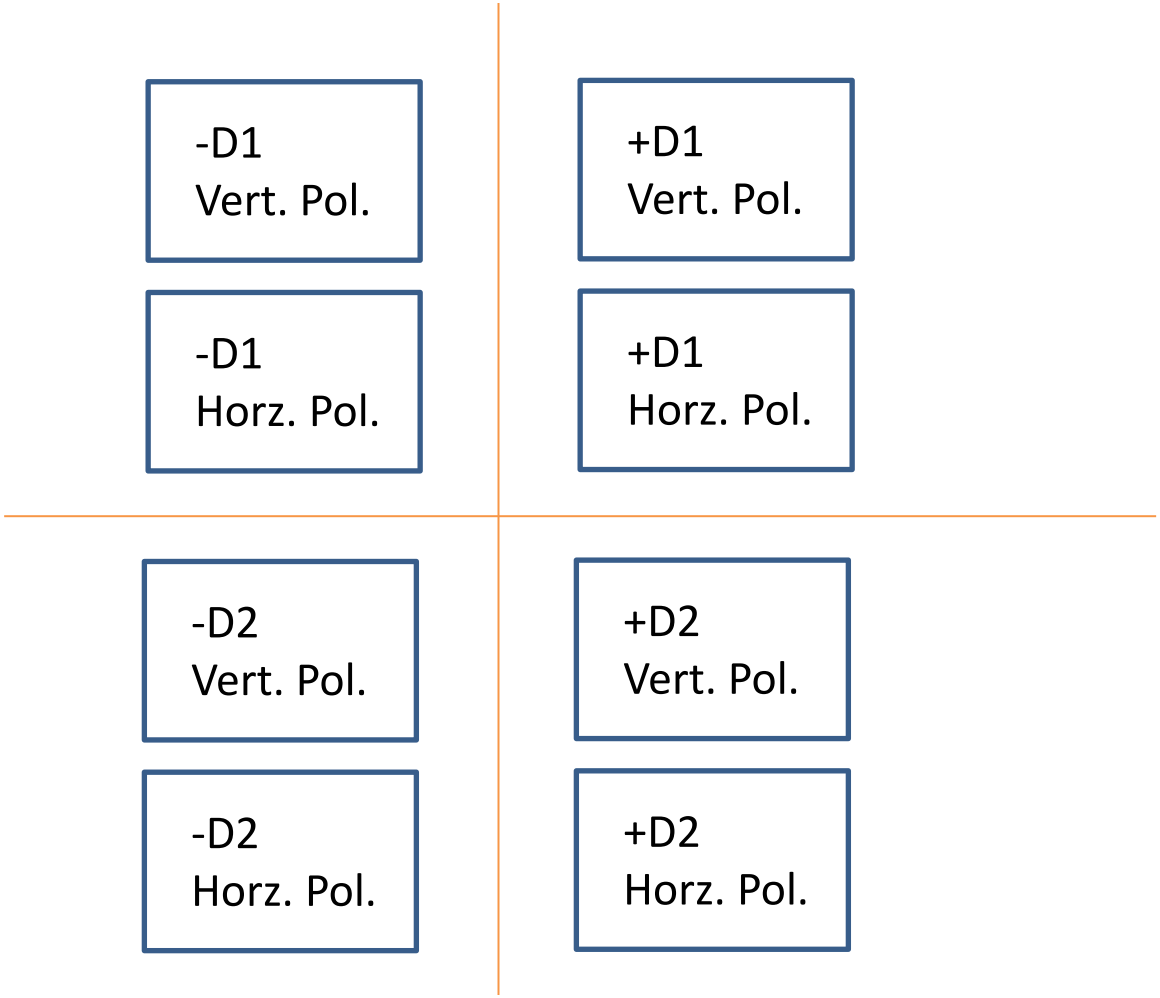

# x=0.1

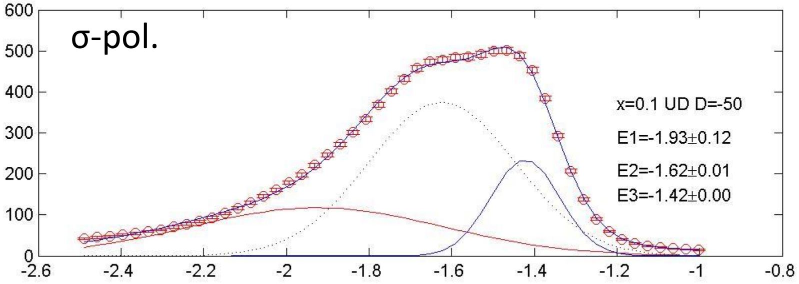
σ-pol.
x=0.1 UD D=-50
E1=-1.93±0.12
E2=-1.62±0.01
E3=-1.42±0.00

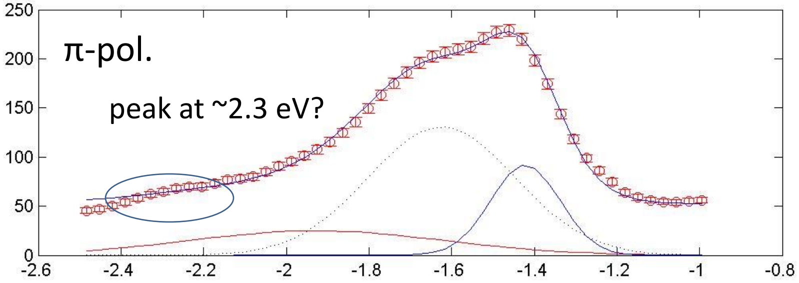
π-pol.
peak at ~2.3 eV?

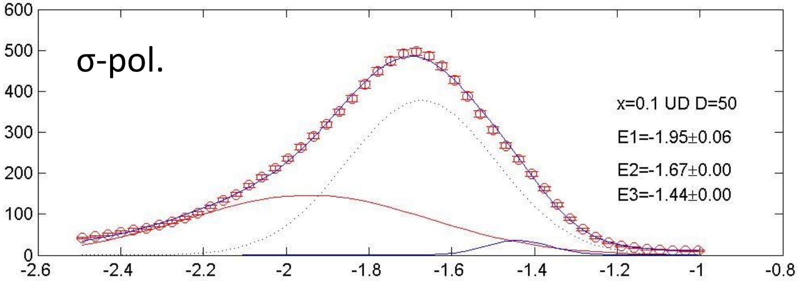
σ-pol.
x=0.1 UD D=50
E1=-1.95±0.06
E2=-1.67±0.00
E3=-1.44±0.00

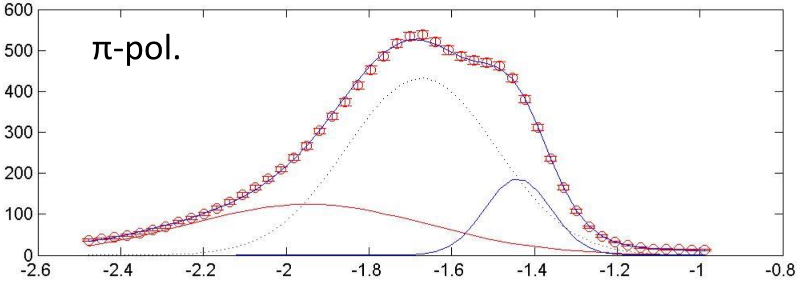
π-pol.

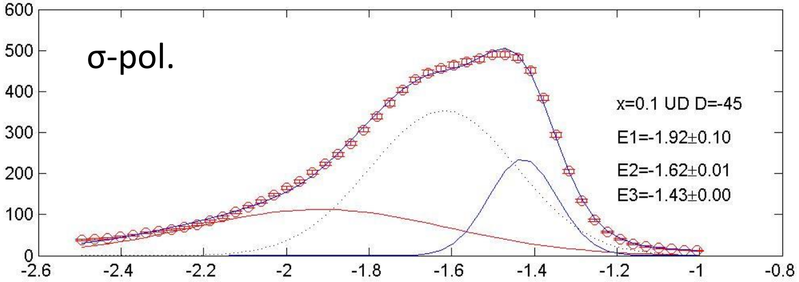
σ-pol.
x=0.1 UD D=-45
E1=-1.92±0.10
E2=-1.62±0.01
E3=-1.43±0.00

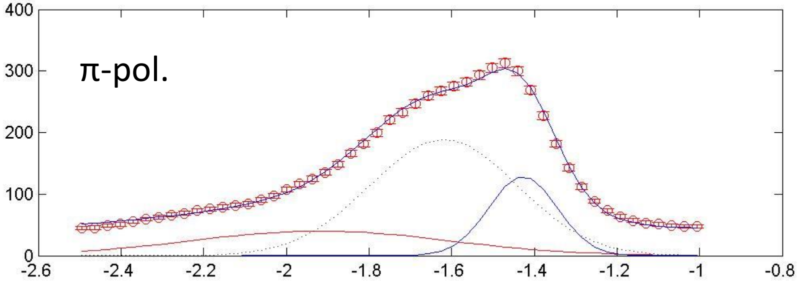
π-pol.

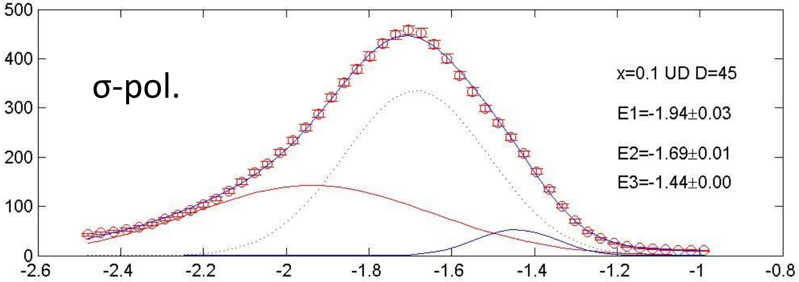
σ-pol.
x=0.1 UD D=45
E1=-1.94±0.03
E2=-1.69±0.01
E3=-1.44±0.00

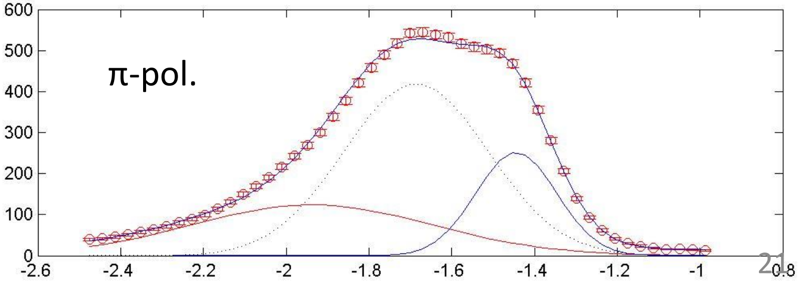
π-pol.

# x=0.1

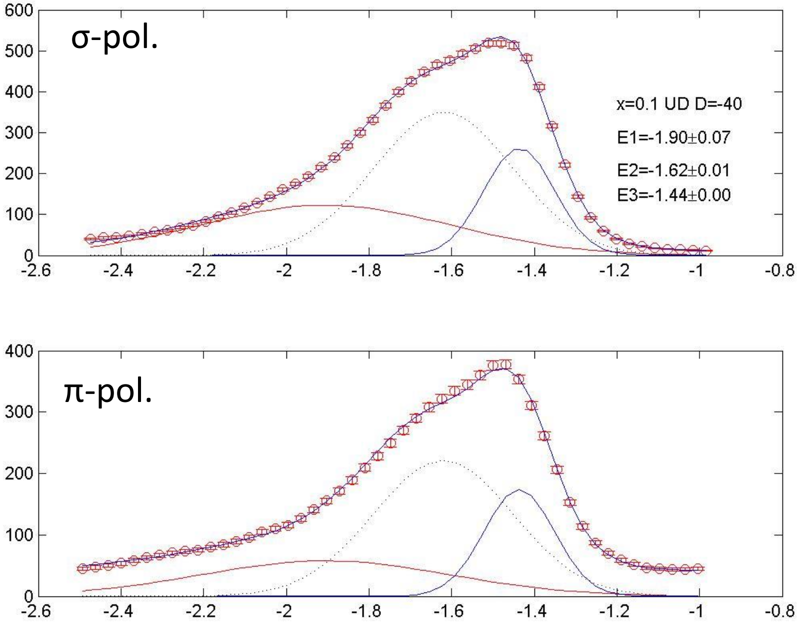
σ-pol.
x=0.1 UD D=-40
E1=-1.90±0.07
E2=-1.62±0.01
E3=-1.44±0.00
π-pol.

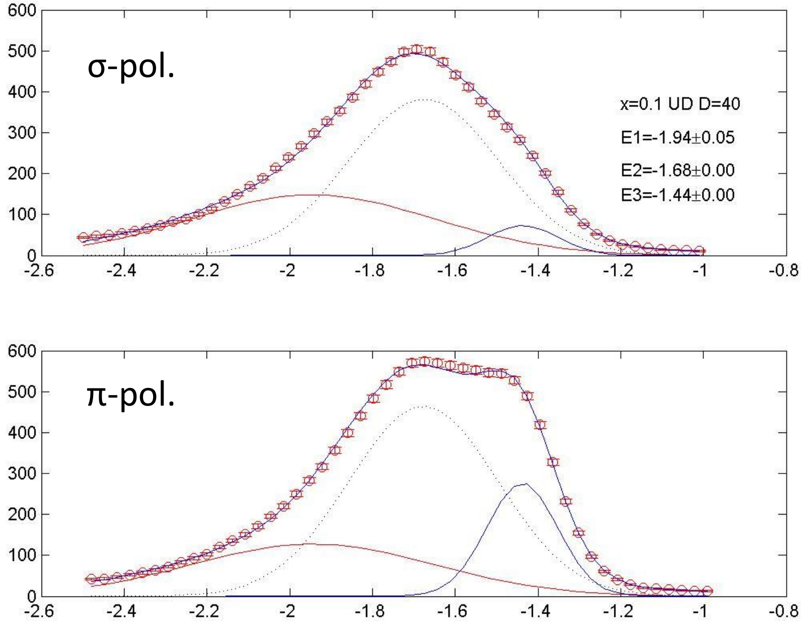
σ-pol.
x=0.1 UD D=40
E1=-1.94±0.05
E2=-1.68±0.00
E3=-1.44±0.00
π-pol.

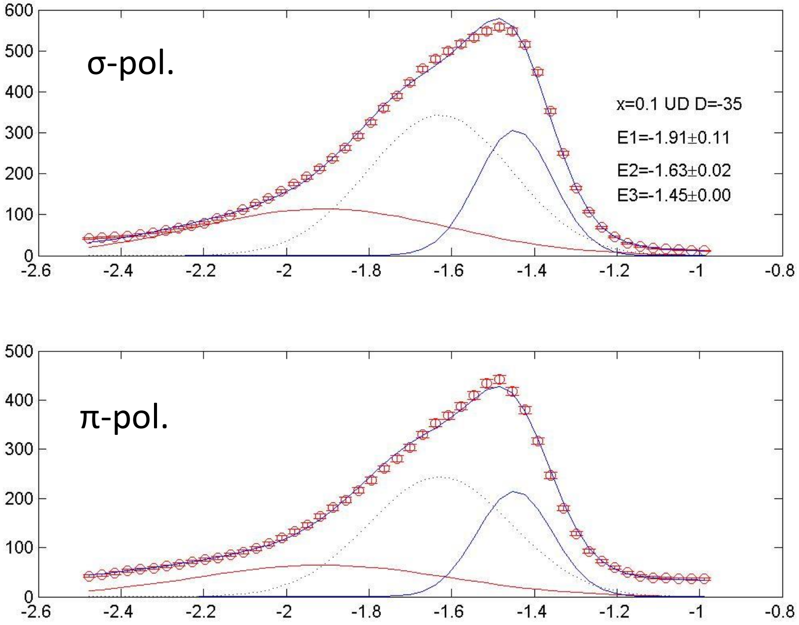
σ-pol.
x=0.1 UD D=-35
E1=-1.91±0.11
E2=-1.63±0.02
E3=-1.45±0.00
π-pol.

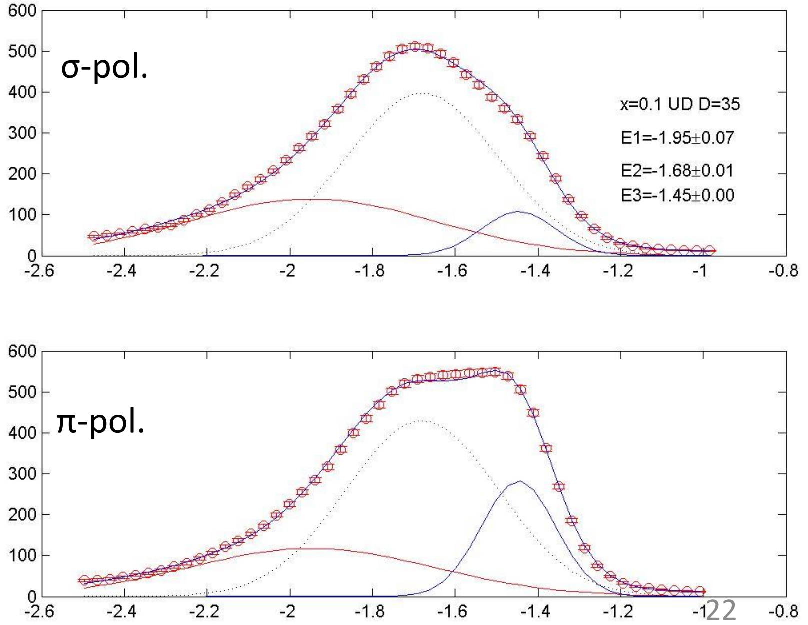
σ-pol.
x=0.1 UD D=35
E1=-1.95±0.07
E2=-1.68±0.01
E3=-1.45±0.00
π-pol.

# x=0.1

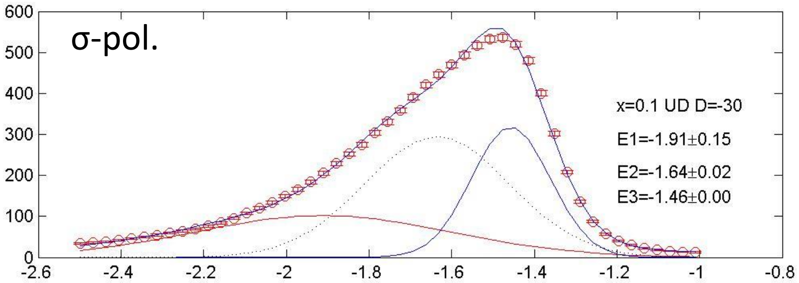
σ-pol.
x=0.1 UD D=-30
E1=-1.91±0.15
E2=-1.64±0.02
E3=-1.46±0.00

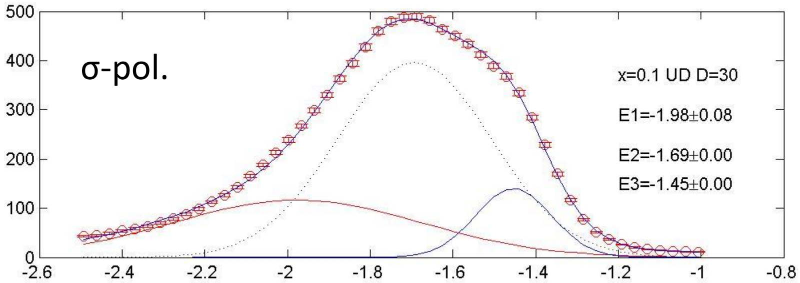
σ-pol.
x=0.1 UD D=30
E1=-1.98±0.08
E2=-1.69±0.00
E3=-1.45±0.00

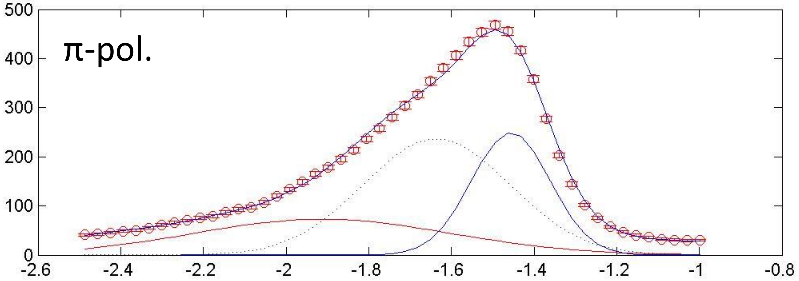
π-pol.

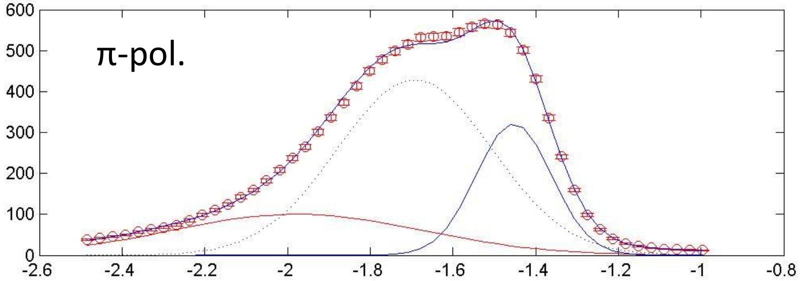
π-pol.

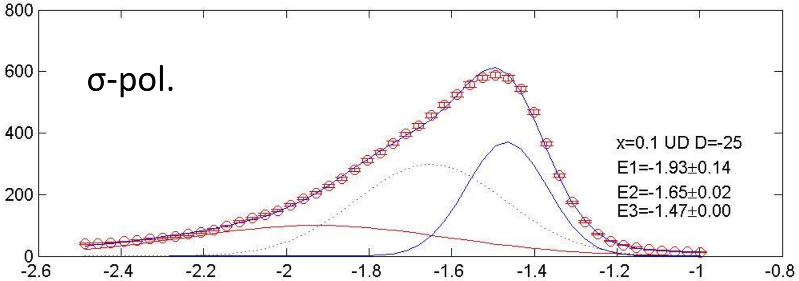
σ-pol.
x=0.1 UD D=-25
E1=-1.93±0.14
E2=-1.65±0.02
E3=-1.47±0.00

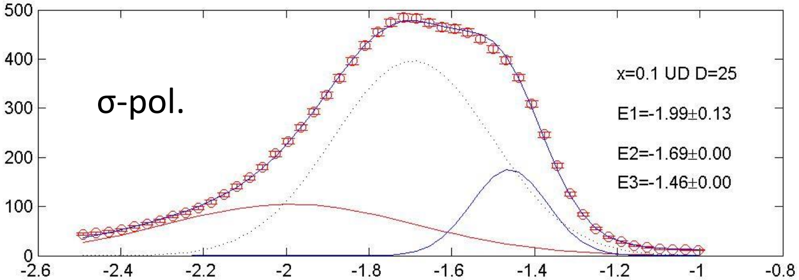
σ-pol.
x=0.1 UD D=25
E1=-1.99±0.13
E2=-1.69±0.00
E3=-1.46±0.00

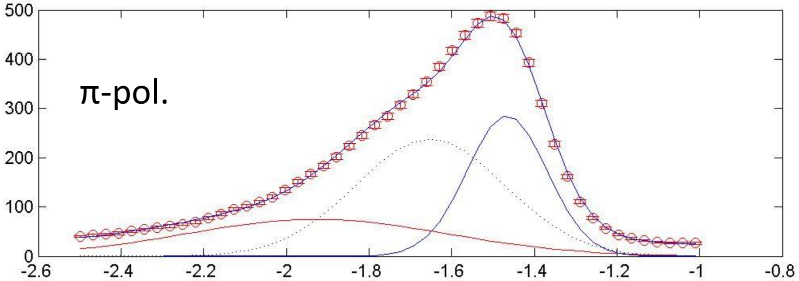
π-pol.

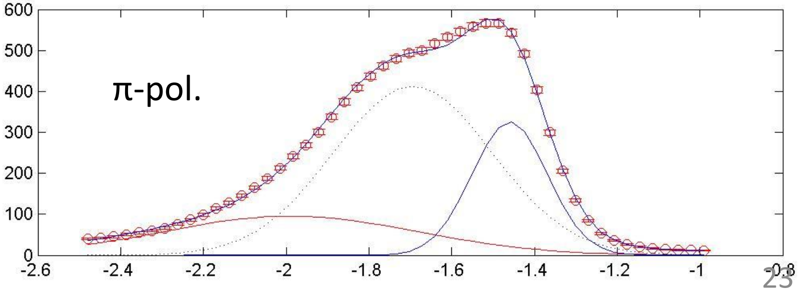
π-pol.

# x=0.1

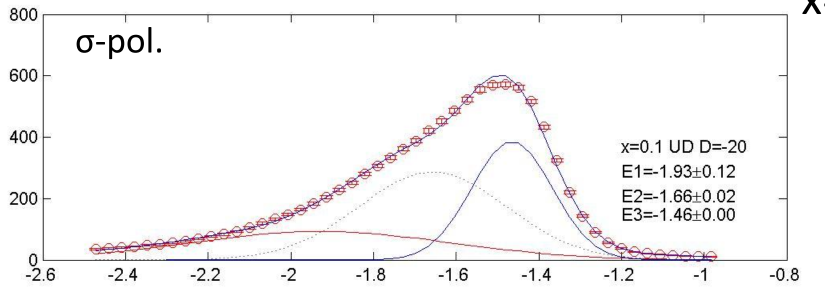
σ-pol.
x=0.1 UD D=-20
E1=-1.93±0.12
E2=-1.66±0.02
E3=-1.46±0.00

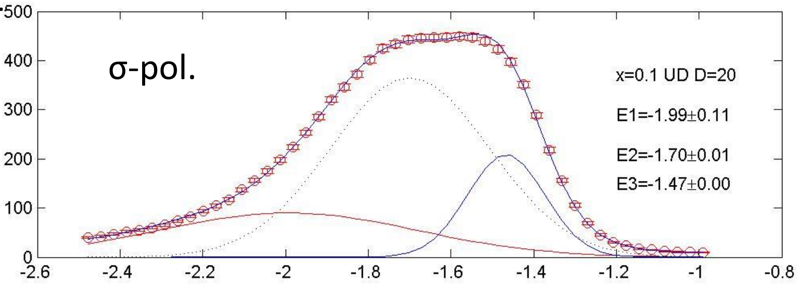
σ-pol.
x=0.1 UD D=20
E1=-1.99±0.11
E2=-1.70±0.01
E3=-1.47±0.00

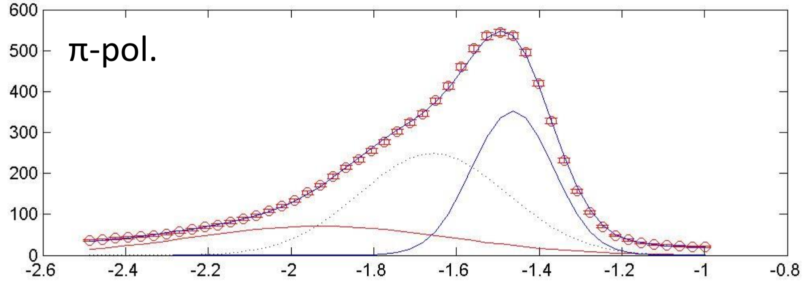
π-pol.

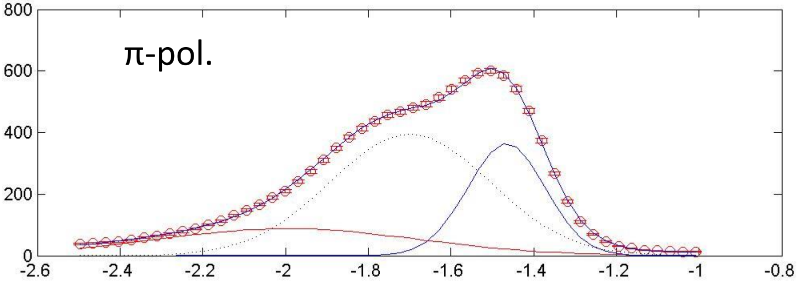
π-pol.

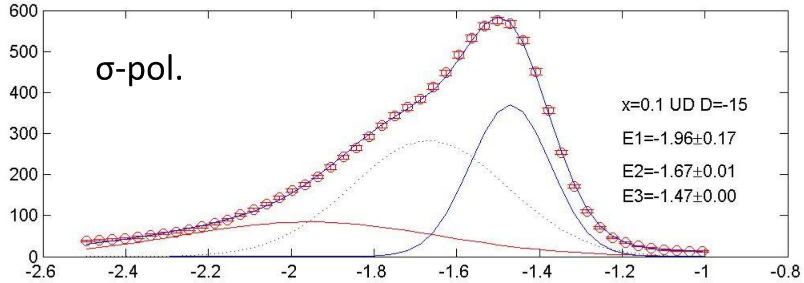
σ-pol.
x=0.1 UD D=-15
E1=-1.96±0.17
E2=-1.67±0.01
E3=-1.47±0.00

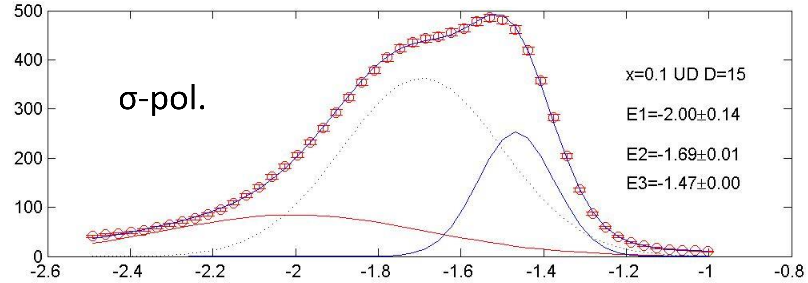
σ-pol.
x=0.1 UD D=15
E1=-2.00±0.14
E2=-1.69±0.01
E3=-1.47±0.00

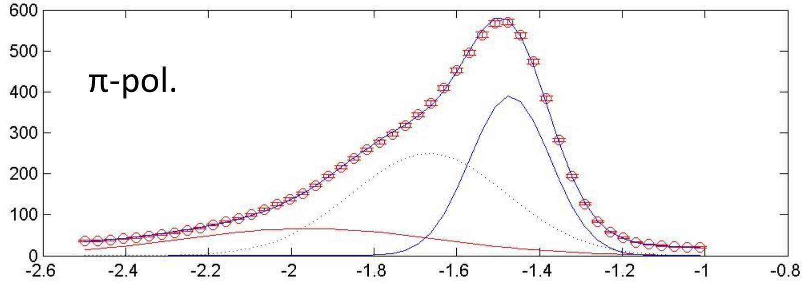
π-pol.

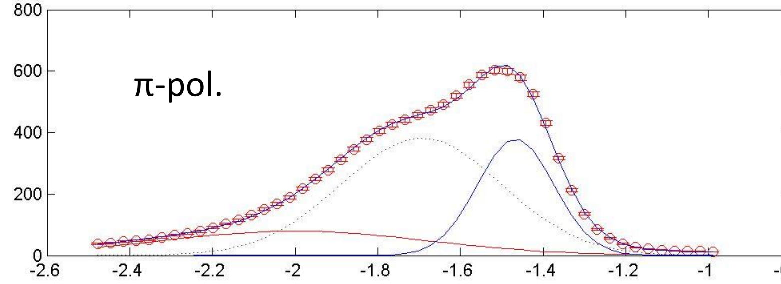
π-pol.

# x=0.1

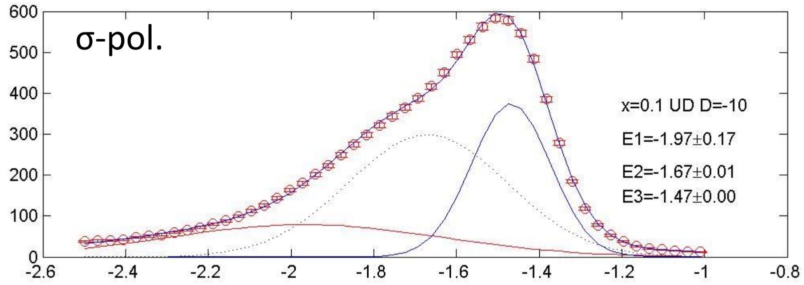
σ-pol.
x=0.1 UD D=-10
E1=-1.97±0.17
E2=-1.67±0.01
E3=-1.47±0.00

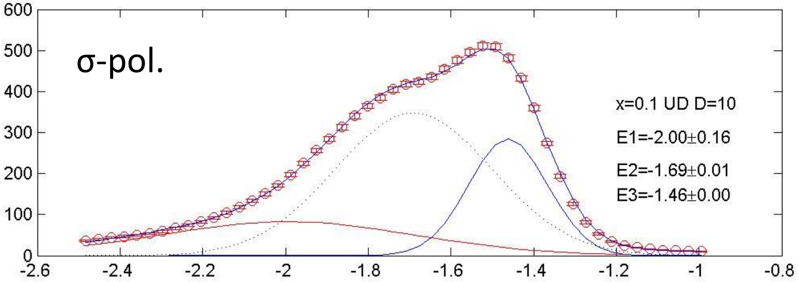
σ-pol.
x=0.1 UD D=10
E1=-2.00±0.16
E2=-1.69±0.01
E3=-1.46±0.00

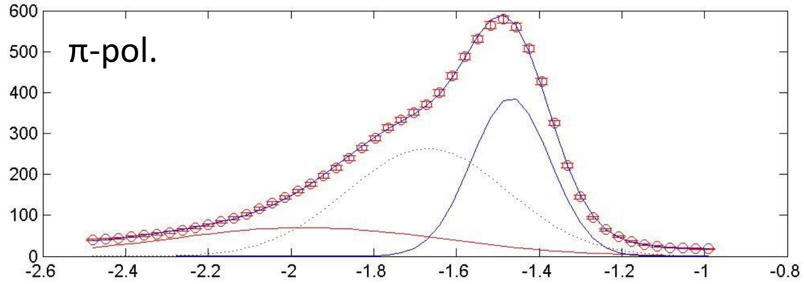
π-pol.

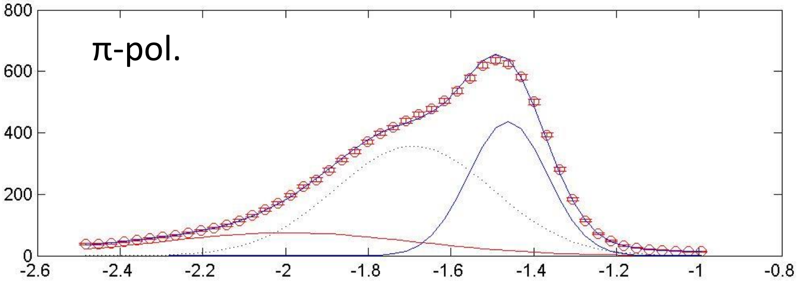
π-pol.

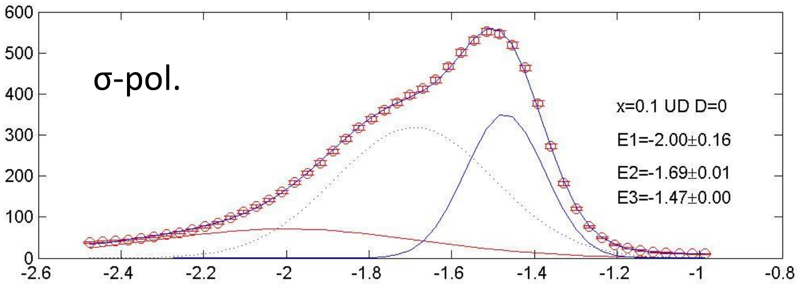
σ-pol.
x=0.1 UD D=0
E1=-2.00±0.16
E2=-1.69±0.01
E3=-1.47±0.00

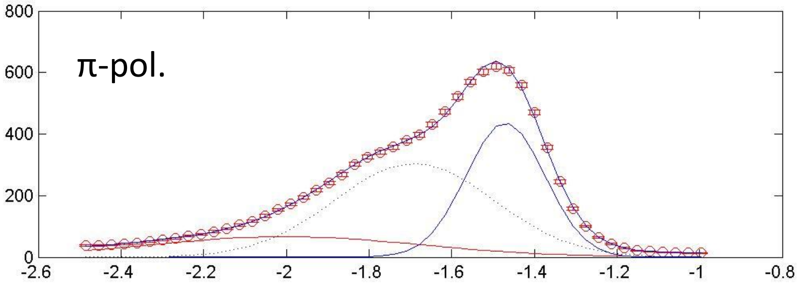
π-pol.

# x=0.4

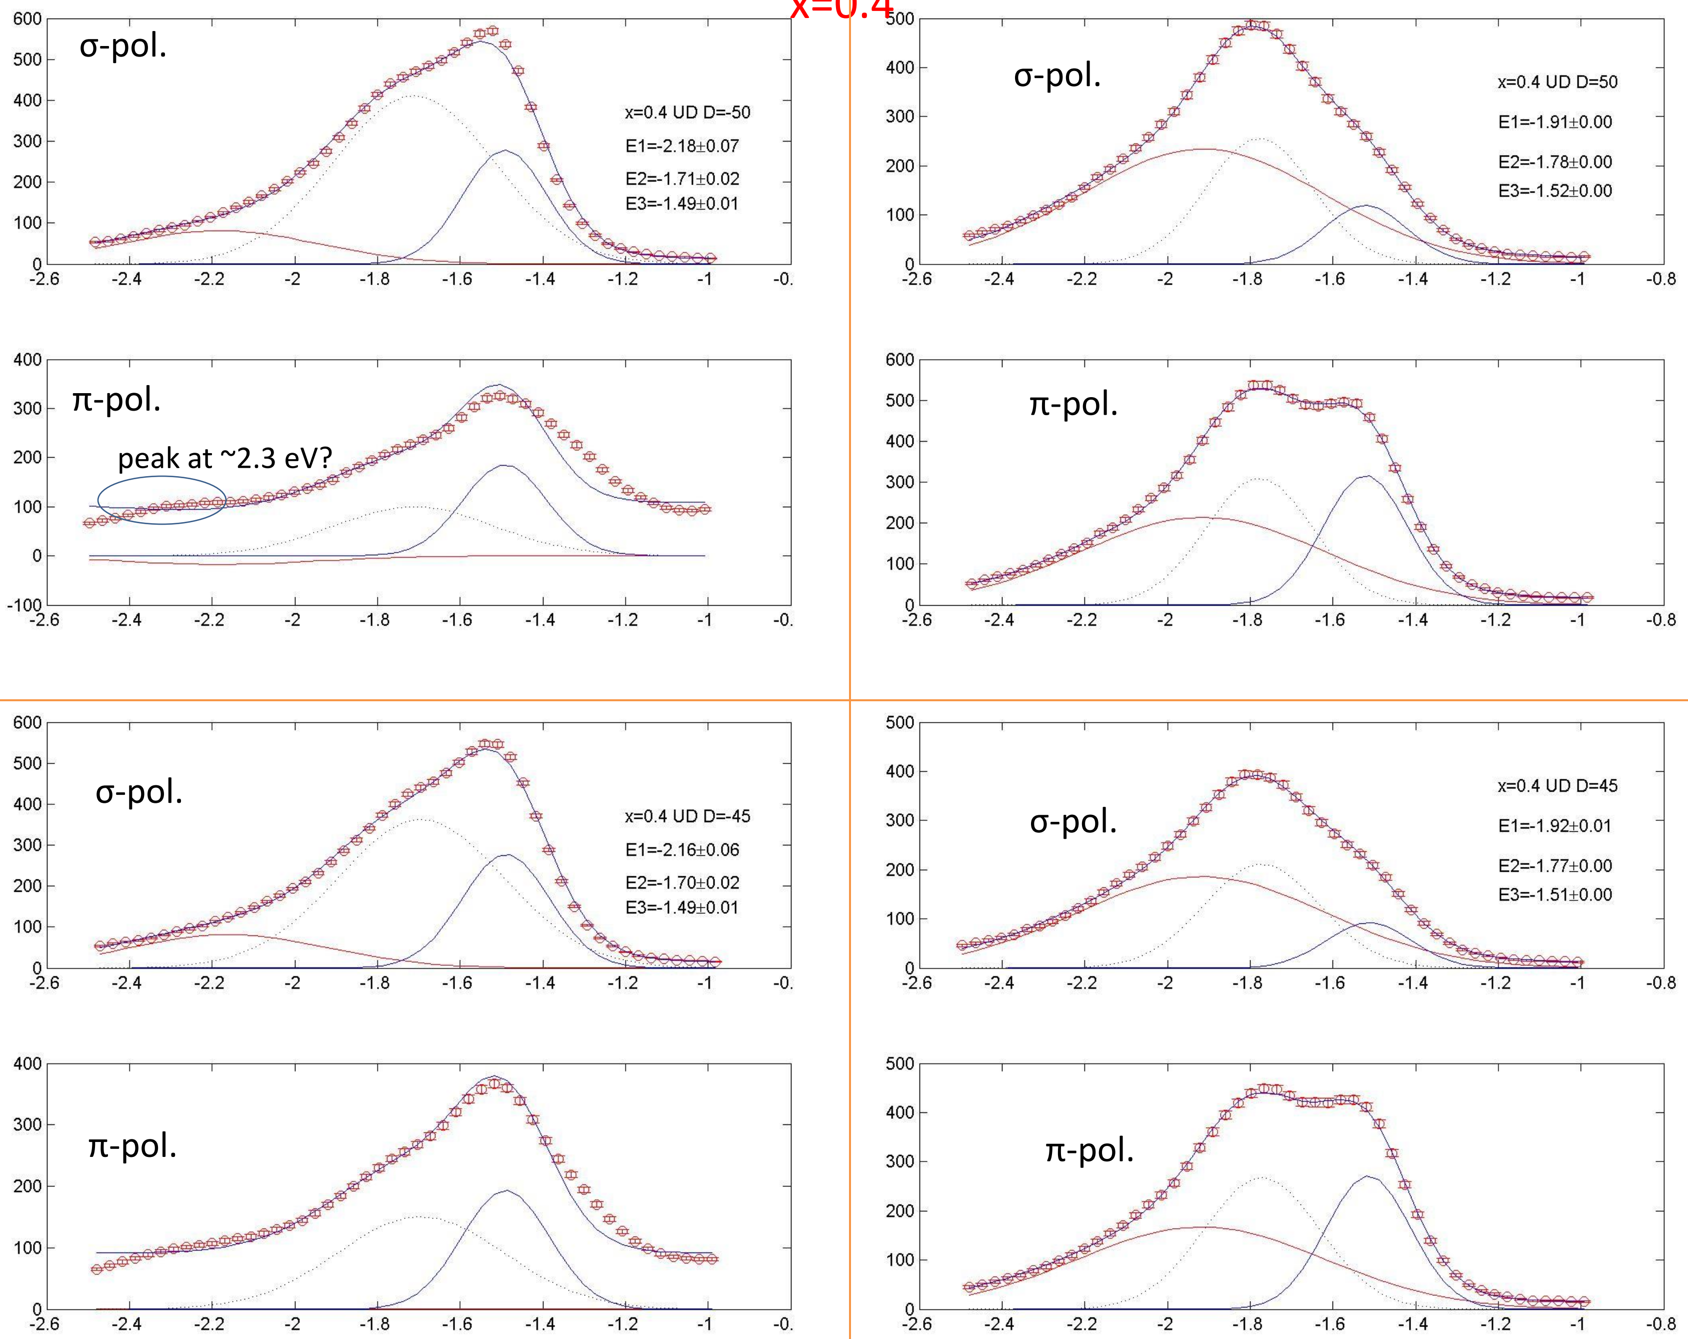

σ-pol.
x=0.4 UD D=-50
E1=-2.18±0.07
E2=-1.71±0.02
E3=-1.49±0.01
π-pol.
peak at ~2.3 eV?
σ-pol.
x=0.4 UD D=50
E1=-1.91±0.00
E2=-1.78±0.00
E3=-1.52±0.00
π-pol.
σ-pol.
x=0.4 UD D=-45
E1=-2.16±0.06
E2=-1.70±0.02
E3=-1.49±0.01
π-pol.
σ-pol.
x=0.4 UD D=45
E1=-1.92±0.01
E2=-1.77±0.00
E3=-1.51±0.00
π-pol.

# x=0.4

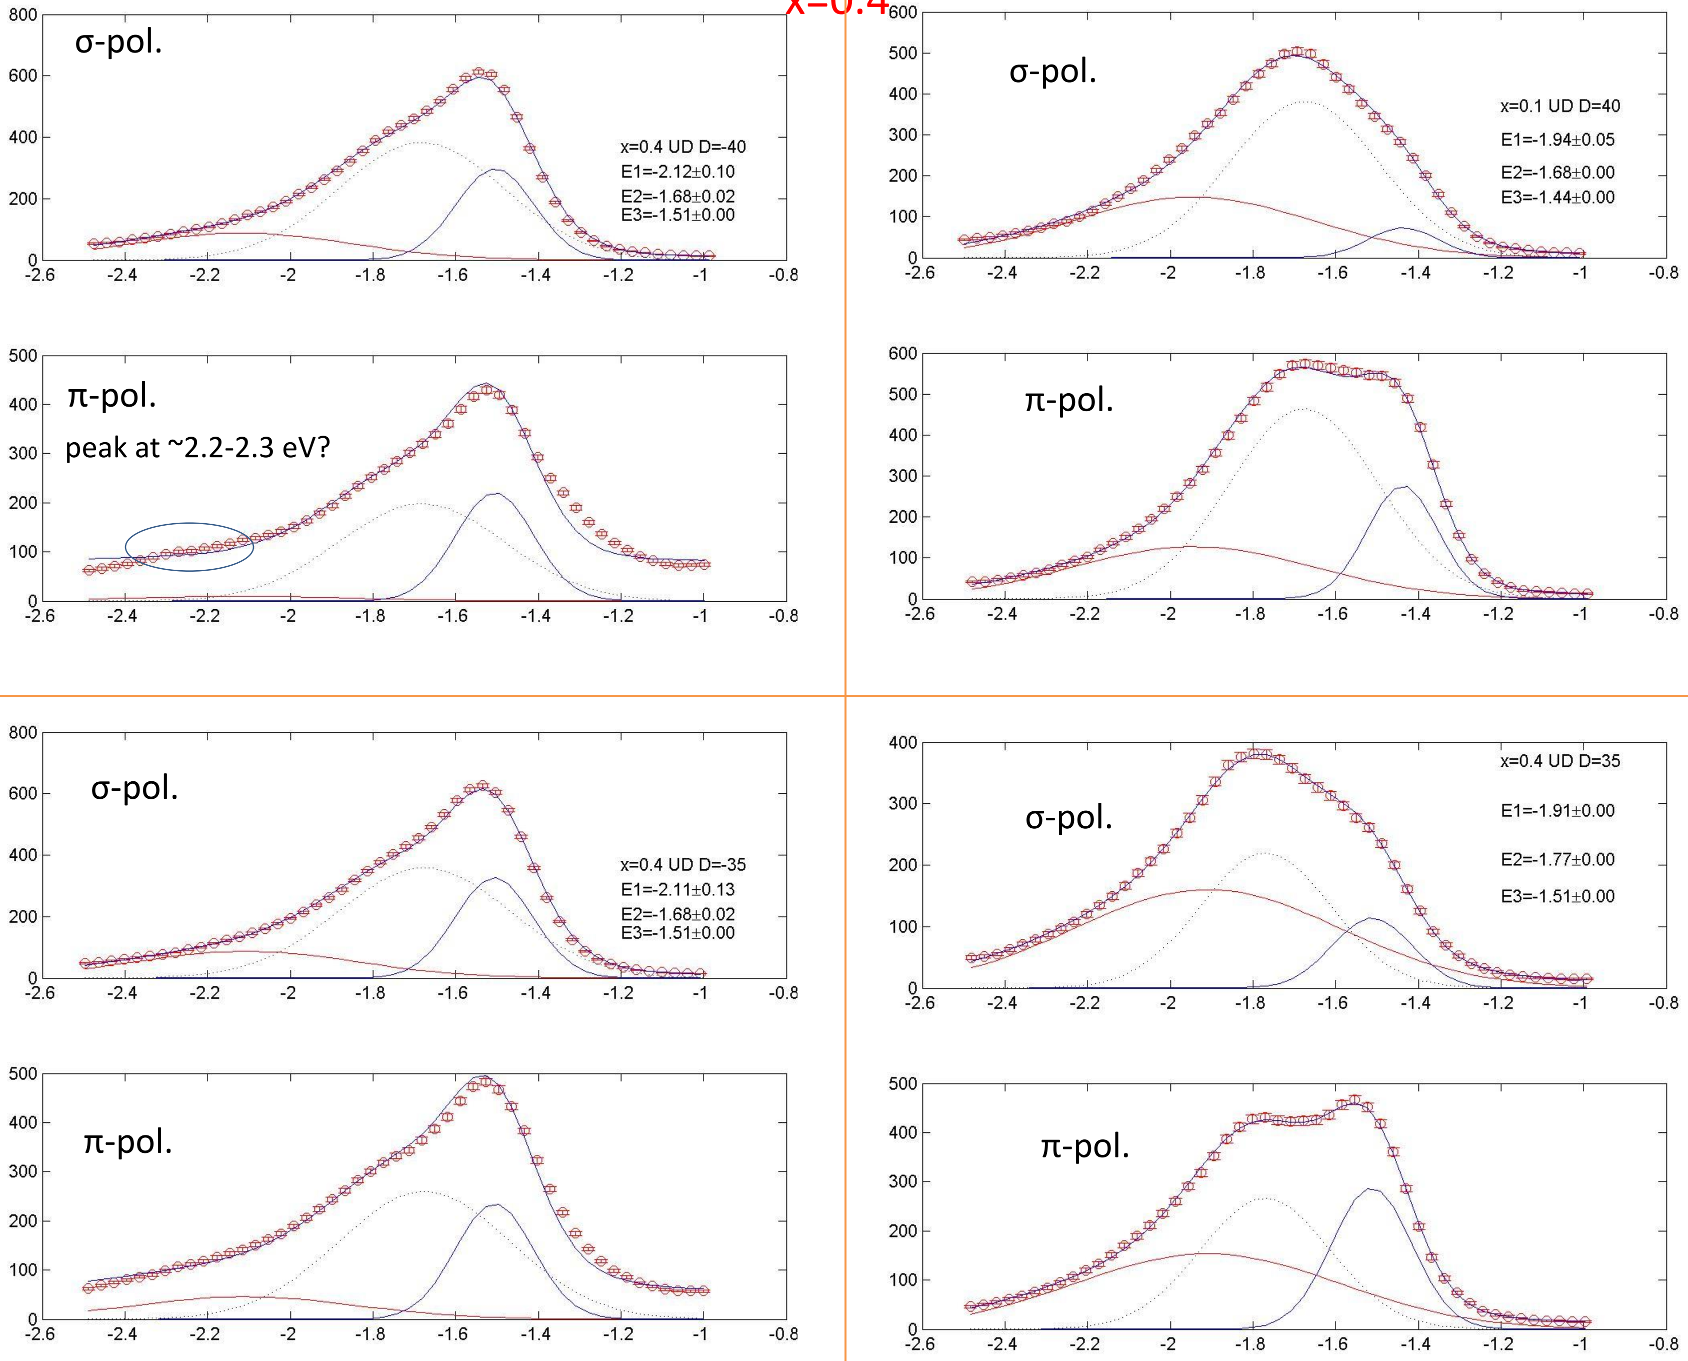

σ-pol.
x=0.4 UD D=-40
E1=-2.12±0.10
E2=-1.68±0.02
E3=-1.51±0.00
π-pol.
peak at ~2.2-2.3 eV?
σ-pol.
x=0.1 UD D=40
E1=-1.94±0.05
E2=-1.68±0.00
E3=-1.44±0.00
π-pol.
σ-pol.
x=0.4 UD D=-35
E1=-2.11±0.13
E2=-1.68±0.02
E3=-1.51±0.00
π-pol.
σ-pol.
x=0.4 UD D=35
E1=-1.91±0.00
E2=-1.77±0.00
E3=-1.51±0.00
π-pol.

x=0.4

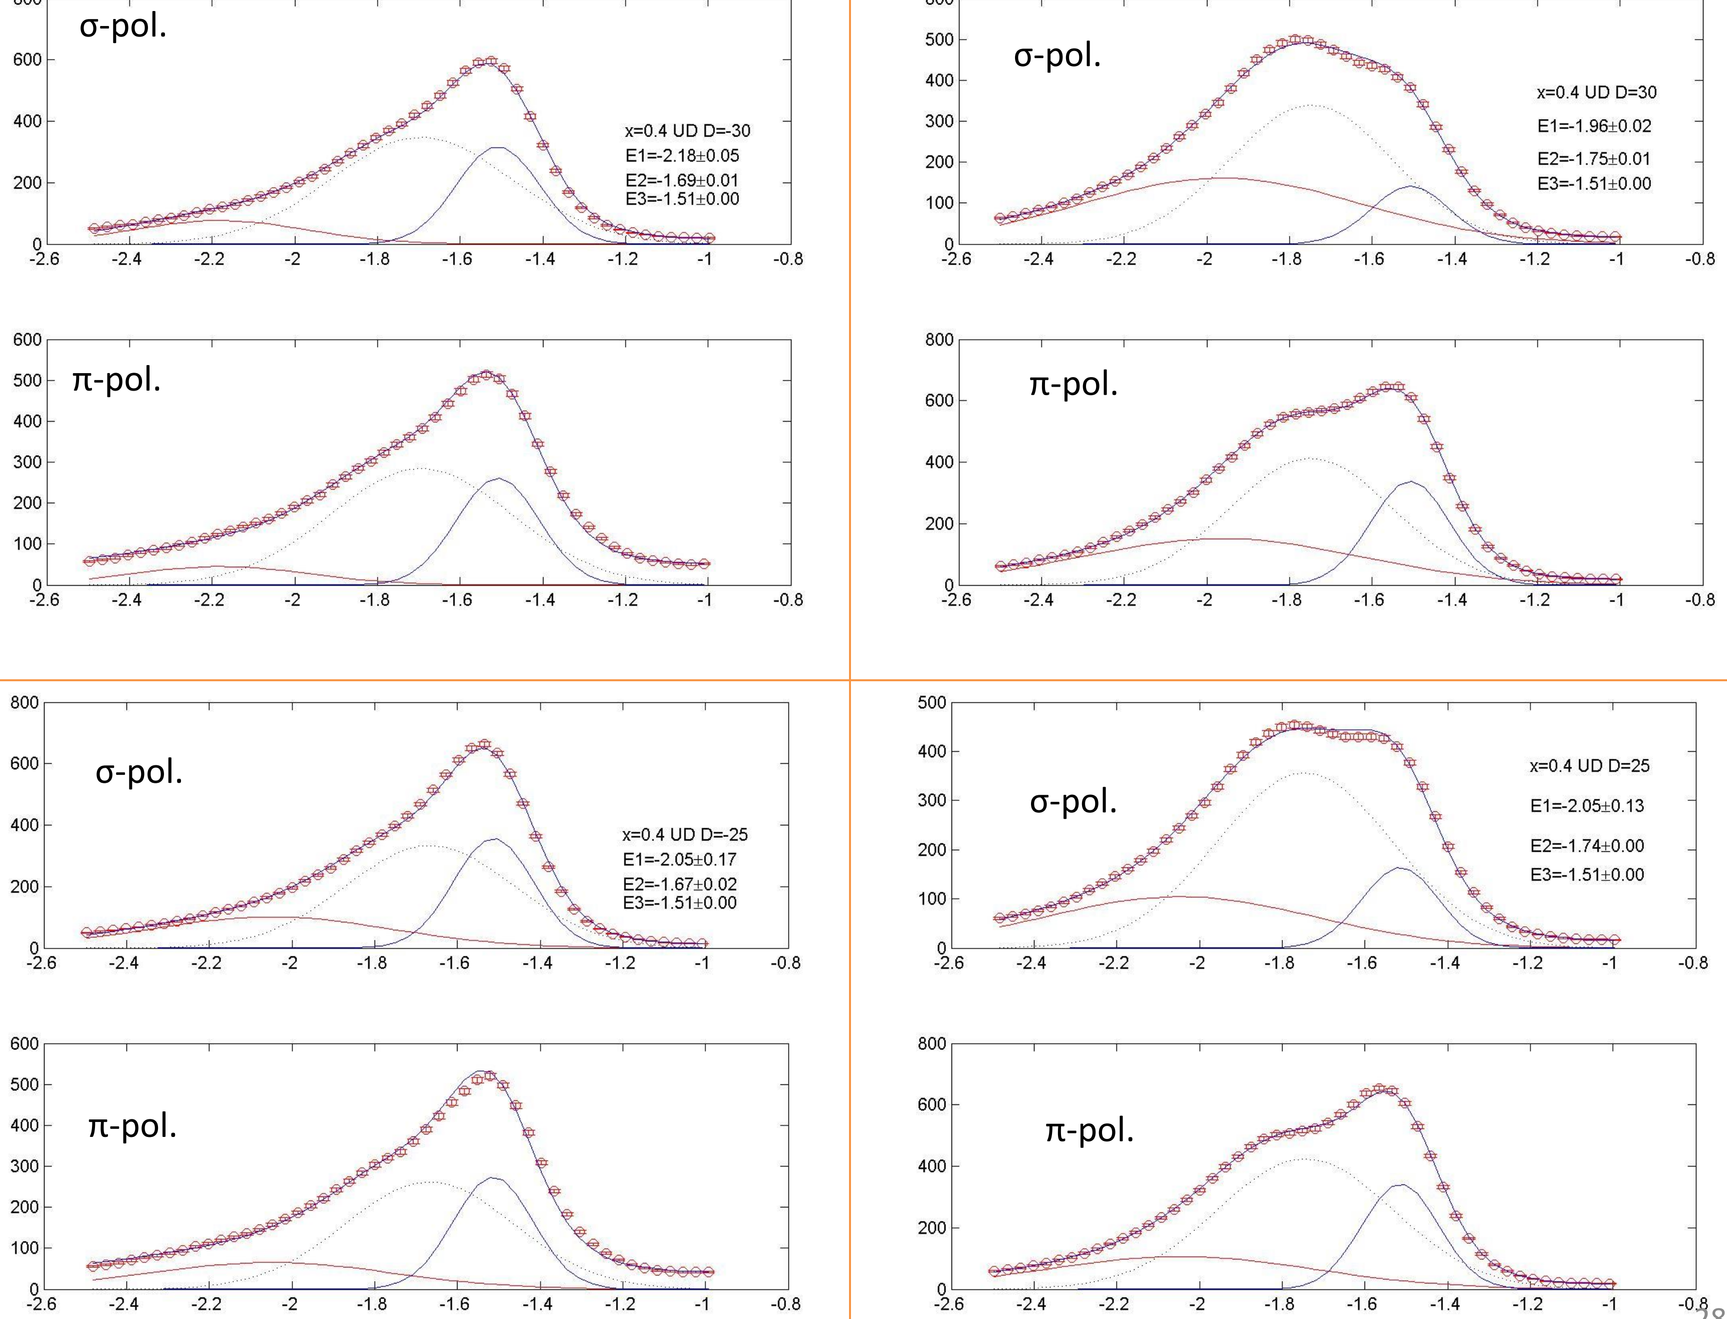
σ-pol.
x=0.4 UD D=-30
E1=-2.18±0.05
E2=-1.69±0.01
E3=-1.51±0.00
π-pol.
σ-pol.
x=0.4 UD D=30
E1=-1.96±0.02
E2=-1.75±0.01
E3=-1.51±0.00
π-pol.
σ-pol.
x=0.4 UD D=-25
E1=-2.05±0.17
E2=-1.67±0.02
E3=-1.51±0.00
π-pol.
σ-pol.
x=0.4 UD D=25
E1=-2.05±0.13
E2=-1.74±0.00
E3=-1.51±0.00
π-pol.

# x=0.4

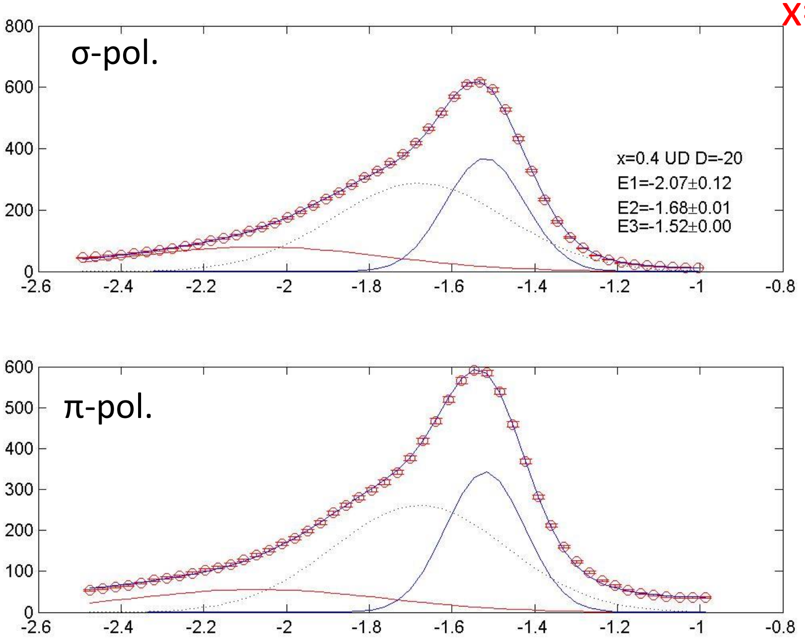
σ-pol.
x=0.4 UD D=-20
E1=-2.07±0.12
E2=-1.68±0.01
E3=-1.52±0.00
π-pol.

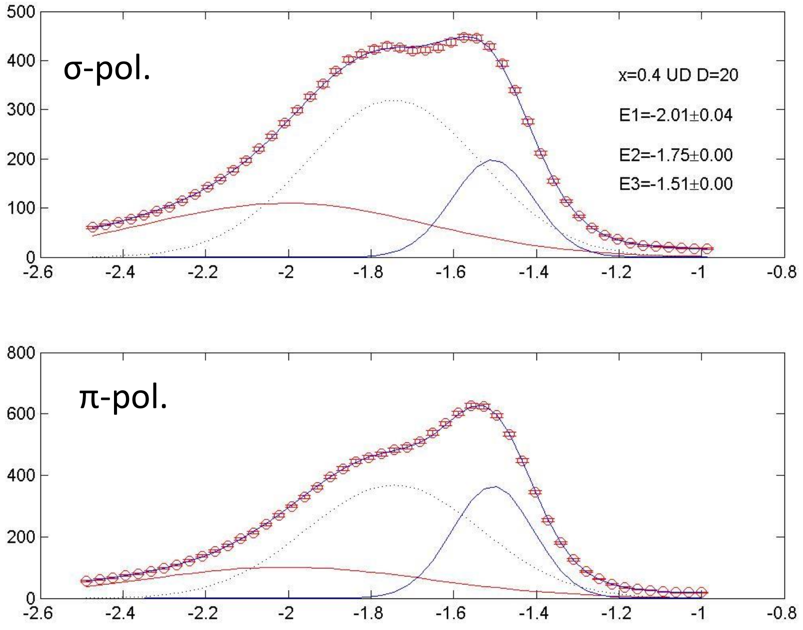
σ-pol.
x=0.4 UD D=20
E1=-2.01±0.04
E2=-1.75±0.00
E3=-1.51±0.00
π-pol.

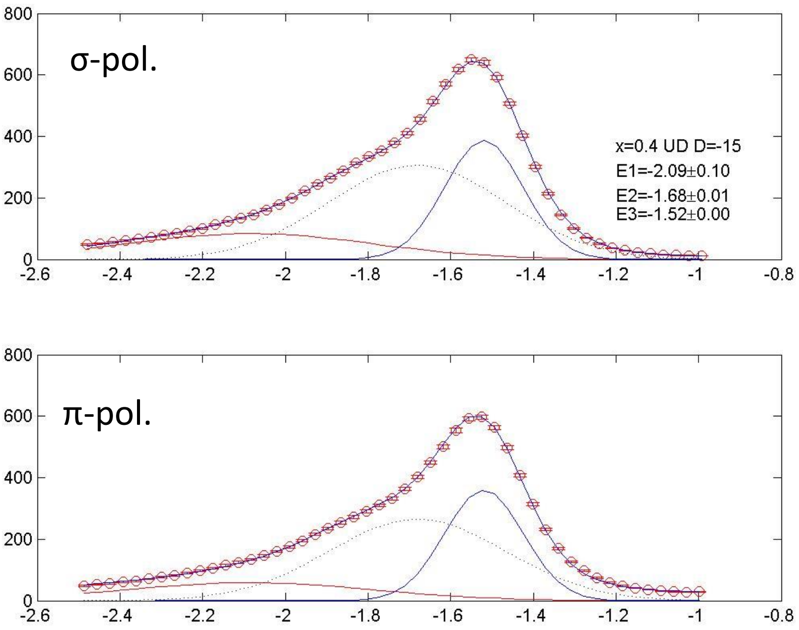
σ-pol.
x=0.4 UD D=-15
E1=-2.09±0.10
E2=-1.68±0.01
E3=-1.52±0.00
π-pol.

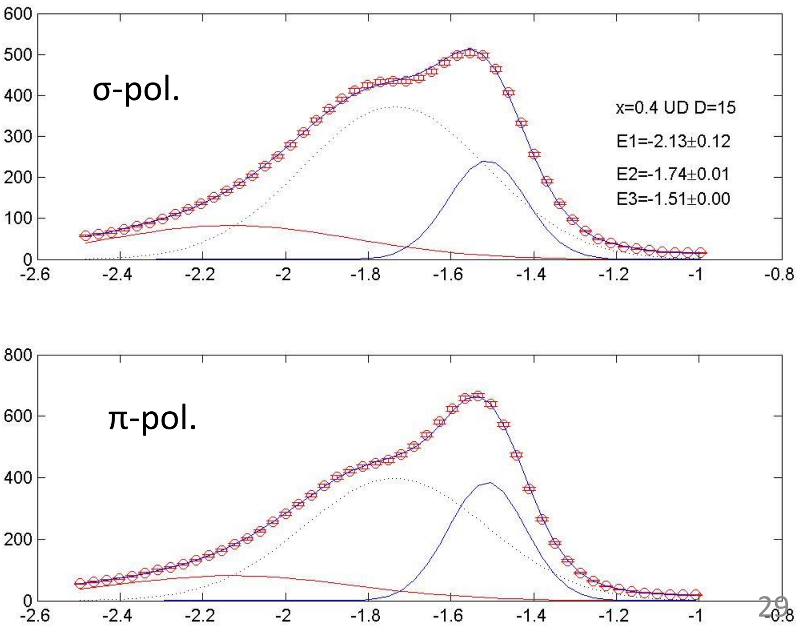
σ-pol.
x=0.4 UD D=15
E1=-2.13±0.12
E2=-1.74±0.01
E3=-1.51±0.00
π-pol.

x=0.4

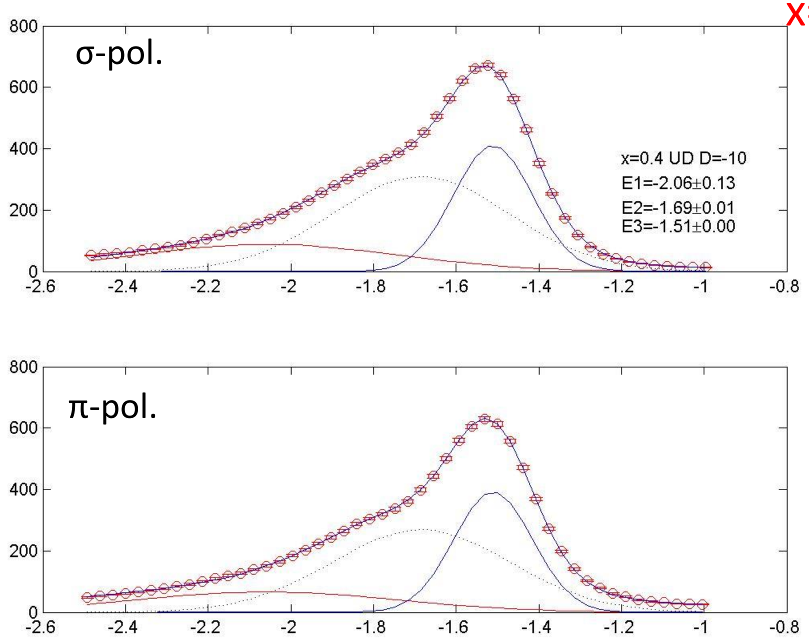
σ-pol.
x=0.4 UD D=-10
E1=-2.06±0.13
E2=-1.69±0.01
E3=-1.51±0.00
π-pol.

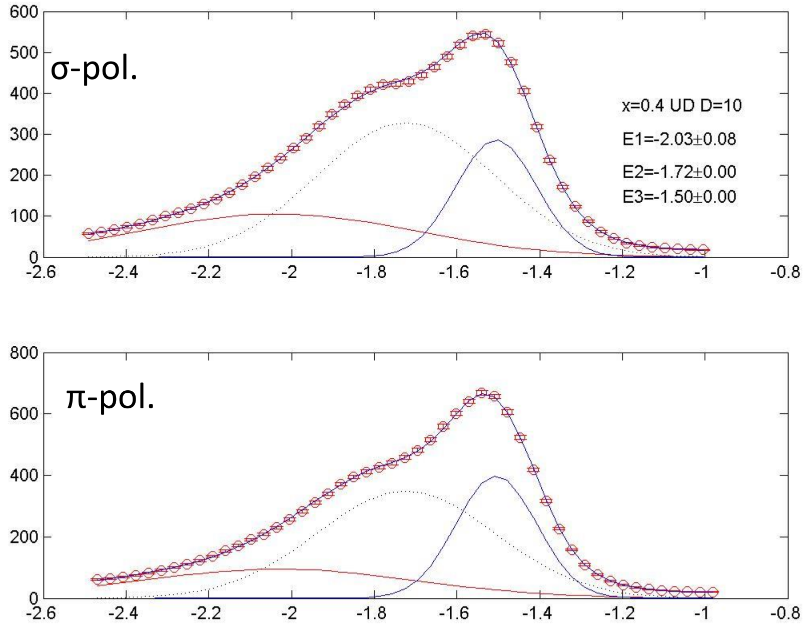
σ-pol.
x=0.4 UD D=10
E1=-2.03±0.08
E2=-1.72±0.00
E3=-1.50±0.00
π-pol.

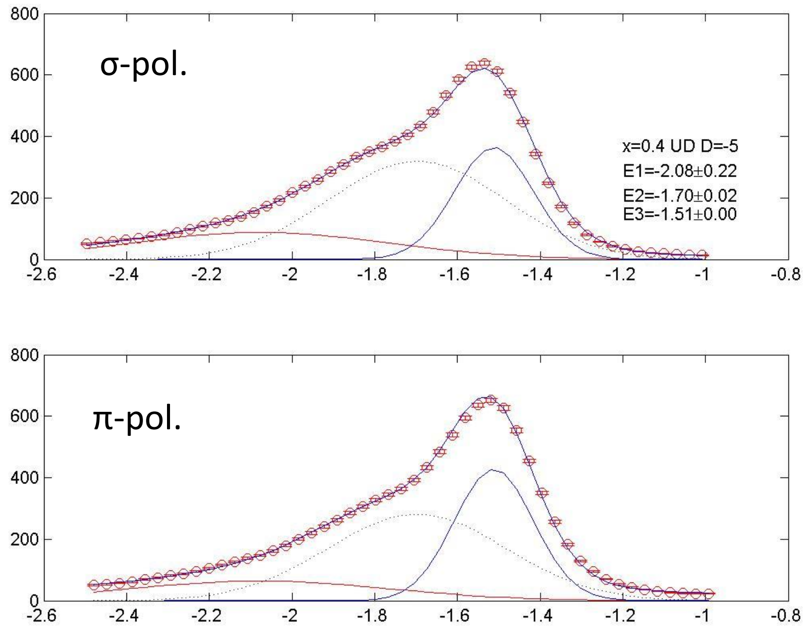
σ-pol.
x=0.4 UD D=-5
E1=-2.08±0.22
E2=-1.70±0.02
E3=-1.51±0.00
π-pol.

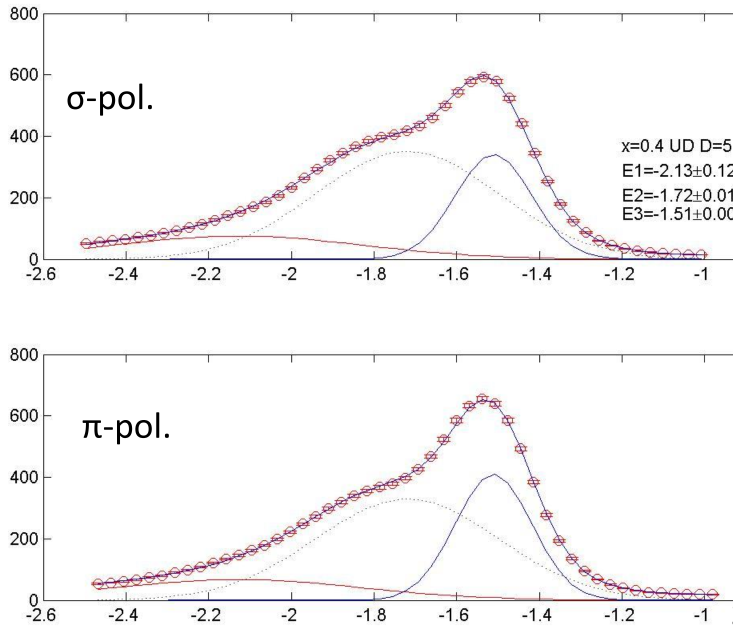
σ-pol.
x=0.4 UD D=5
E1=-2.13±0.12
E2=-1.72±0.01
E3=-1.51±0.00
π-pol.

# x=0.4

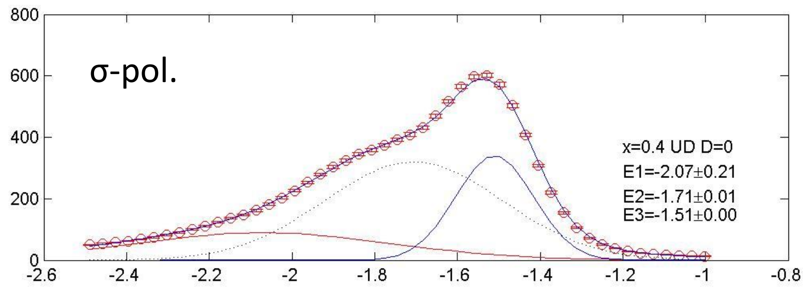


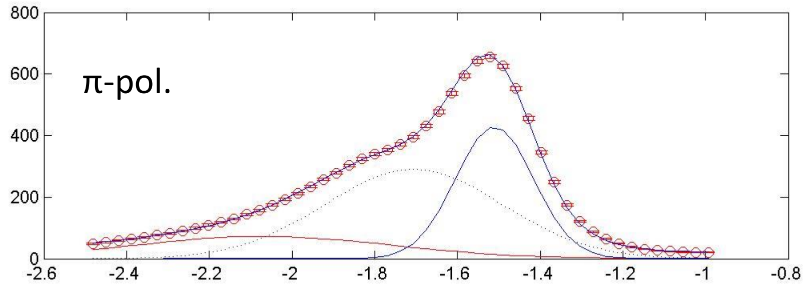

Supplement: Supplementary file 1 [file supplementary_june2015.pdf]
